# Supplementary material for: Conversion rules for Weyl points and nodal lines in topological media
Source: arXiv:1803.06364 ancillary file (2018-09-05)
Supplement: Supplementary file 1 [file Supplementary_material.pdf]

# Supplemental material for:
# Conversion rules for Weyl points and nodal lines in topological media

Xiao-Qi Sun,[1,2] Tomáš Bzdušek,[1,2] and Shou-Cheng Zhang[1,2]

[1]*Department of Physics, McCullough Building, Stanford University, Stanford, California 94305-4045, USA*
[2]*Stanford Center for Topological Quantum Physics, Stanford University, Stanford, California 94305-4045, USA*

## CONTENTS

I. Introduction ii

II. Relative homotopy theory ii
A. Formal definition of homotopy groups ii
B. Relative homotopy groups iii
C. Long exact sequence of homotopy classes iv

III. Analysis of band-structure nodes vi
A. General strategy vii
B. Nodal class A with mirror viii
C. Nodal class A with $C_{2z}\mathcal{T}$ x
D. Nodal class C with $C_{2z}\mathcal{T}$ x

IV. Lattice models xiii
A. Lattice model for the topologically non-trivial nodal loop on a mirror invariant plane xiii
B. Lattice model for the topologically non-trivial nodal-chain in the presence of two mirror symmetries xiv
C. Lattice model exhibiting the conversion of Weyl points in the presence of $C_{2z}\mathcal{T}$ symmetry xvi

V. No stable Fermi arcs for nodes in systems with $(\mathcal{PT})^2 = +\mathbf{1}$ symmetry xvi

VI. Generalization to multi-band models xviii

References xix

# I. INTRODUCTION

In the main text, we introduced new topological crystalline invariants following from relative homotopy groups of the space of Hamiltonians. Specifically, we discussed the new invariants appearing in two-band models with mirror or $C_{2z}\mathcal{T}$ symmetry. In the presence of a mirror symmetry, we established a novel nodal line phases that exhibits both Fermi arcs and drumhead states on the surface. Such nodal lines convert into a residual pair of Weyl points (WPs) when shrunk. We further showed that in systems with a pair of mirror symmetries, multiple nodal lines in two mirror-invariant planes can combine into a nodal chain which exhibits multiple surface Fermi arcs. These nodal chains can be converted into quadruple WPs. Finally, we established conversion rules for WPs in systems with $C_{2z}\mathcal{T}$ symmetry.

In this supplementary material, we provide additional information to strengthen our claims. We begin in Sec. II with a review of homotopy theory that we use to describe band-structure nodes. In Sec. III, we use homotopy theory to explicitly derive the new topological invariants in the presence of mirror or $C_{2z}\mathcal{T}$ symmetry. Besides the semimetallic systems considered in the main text, we also explicitly consider an class of superconducting models for which a non-trivial conversion rule survives in the presence of multiple bands. We continue in Sec. IV with a discussion of the two-band lattice Hamiltonians used to plot the figures in the main text. These include the Hamiltonian with one (two) mirror symmetries or with $C_{2z}\mathcal{T}$ symmetry. In Sec. V, we comment on the absence of surface Fermi arcs in nodal-line semimetals with a non-trivial monopole charge, which exists in the presence of $(\mathcal{PT})^2 = +\mathbf{1}$. Finally, we clarify in Sec. VI how the conversions derived for two-band semimetallic models change in the presence of additional bands. Specifically, we discuss how the conversion following from a mirror symmetry is modified if the additional bands are only weakly coupled to the original two bands.

# II. RELATIVE HOMOTOPY THEORY

In this section, we review homotopy theory needed in our description of band-structure nodes. We begin in Sec. II A with a discussion of homotopy groups, and continue in Sec. II B with an overview of relative homotopy groups. Finally, in Sec. II C we show how one can derive the latter from the first using a long exact sequence of homomorphisms between these groups. Our discussion is largely based on in Refs. [1] and [2].

## A. Formal definition of homotopy groups

We aim to study *continuous maps* $f$ from a *p-dimensional sphere* $S^p$ (with $p$ a *non-negative integer*, and where $S^0$ corresponds to an ordered union of two points) to a *topological space* $M$. Especially, we might wonder whether two such maps $f_1$ and $f_2$ can be transformed into each other with continuous deformations. As explained in the main text, such considerations lie at the core of the classification of band-structure nodes protected by local-in-$\mathbf{k}$ symmetries [3]. An analogous analysis has been previously applied to the classification of defects in ordered media [2].

One can introduce a group structure into the space of such continuous maps for $p \geq 1$ if we further require a selected point $\mathrm{P} \in S^p$ (e.g. the "north pole") to be mapped to a *base point* $\mathfrak{m} \in M$. We call such maps as *pointed*. The resulting group does not depend on the specific choice of $\mathfrak{m}$ if $M$ is *connected* [1]. To uncover the group structure, it is convenient to "punch a hole" at P and to stretch $S^p\backslash\{\mathrm{P}\}$ into a *p-dimensional hypercube* $[0,1]^p \equiv I^p$, which effectively inflates the point P to the *boundary* $\partial I^p$. The considered maps on $S^p$ are thus transformed into continuous maps fulfilling

$$f: \begin{array}{ccc} I^p & \to & M \\ \partial I^p & \to & \mathfrak{m}. \end{array} \tag{1}$$

The space $\widetilde{\pi}_p(M,\mathfrak{m})$ of *all* continuous maps fulfilling conditions (1) is closed under the binary composition "$\circ$" defined by

$$(f_1 \circ f_2)(x_1, x_2, \ldots, x_p) := \begin{cases} f_1(2x_1, x_2, \ldots, x_p) & \text{for } 0 \leq x_1 \leq \frac{1}{2} \\ f_2(2x_1 - 2, x_2, \ldots, x_p) & \text{for } \frac{1}{2} < x_1 \leq 1 \end{cases} \tag{2}$$

where $(x_1, \ldots, x_p) = \mathbf{x}$ are coordinates running along the edges of $I^p$. However, there is no identity element $e \in \widetilde{\pi}_p(M,\mathfrak{m})$ for operation "$\circ$", such that $f \circ e = f = e \circ f$ for all $f$ satisfying (2). The absence of the identity element means that $\widetilde{\pi}(M,\mathfrak{m})$ is just a *semigroup*.

One can avoid this problem by instead considering the set $\pi_p(M,\mathfrak{m})$ of *equivalence classes* of maps that can be continuously deformed into one another while preserving conditions (1). We write $[f]$ to represent the equivalence class of maps reachable from $f$ in this way. Maps $f_1$ and $f_2$ are *equivalent* if there exists a *homotopy* $\mathcal{F}: I^p \times I \to M$ that continuously interpolates $f_1$ and $f_2$, i.e. a continuous map such that $\forall \mathbf{x} \in I^p$ and $\forall t \in I$:

$$\mathcal{F}(\mathbf{x},0) = f_1(\mathbf{x}), \qquad \mathcal{F}(\mathbf{x},1) = f_2(\mathbf{x}) \qquad \text{and} \qquad \mathcal{F}(\partial I^p, t) = \mathfrak{m}. \tag{3}$$

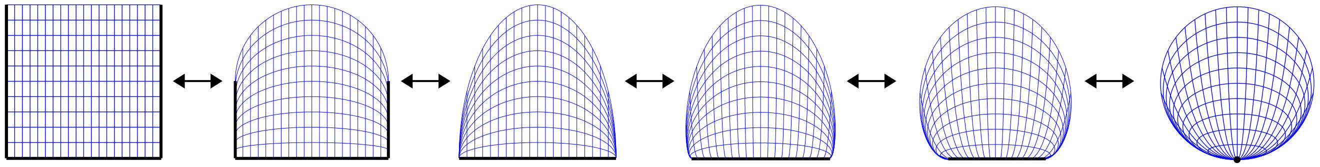

**Figure** S-1. We begin with $I^p$ for which all but one face ($x_p = 1$) are mapped to the base point $\mathfrak{m}$ (indicated by black lines). The hypercube is then continuously deformed into $D^p$ with a only single point on the boundary mapped to $\mathfrak{m}$. The illustration corresponds to $p = 2$, but the concept easily generalizes to $p \geq 3$.

If we interpret the second argument as time, $\mathcal{F}$ evolves $f_1$ to $f_2$ while respecting conditions (1). Clearly, $[f_1] = [f_2]$ whenever $f_1$ and $f_2$ are equivalent. We can then define the binary operation "$\circ$" on $\pi_p(M, \mathfrak{m})$ by

$$[f_1] \circ [f_2] := [f_1 \circ f_2]. \tag{4}$$

It is easy to see that if $f_\mathfrak{m} : I^p \to \mathfrak{m}$ is the constant map, then

$$[f] \circ [f_\mathfrak{m}] = [f] \quad \text{with homotopy} \quad \mathcal{F}(x_1, x_2, \ldots, x_p, t) = \begin{cases} f(\frac{2}{1+t}x_1, x_2, \ldots, x_p) & \text{for } x_1 \leq \frac{1+t}{2} \\ \mathfrak{m} \quad \text{otherwise} \end{cases} \tag{5}$$

(and similarly $[f_\mathfrak{m}] \circ [f] = [f]$), implying that $[f_\mathfrak{m}]$ is the identity element of "$\circ$" in $\pi_p(M, \mathfrak{m})$. Furthermore, the map

$$f^{-1}(x_1, x_2, \ldots, x_p) := f(1 - x_1, x_2, \ldots, x_p) \tag{6}$$

fulfils

$$[f] \circ [f^{-1}] = [f_\mathfrak{m}] \quad \text{with homotopy} \quad \mathcal{F}(x_1, x_2, \ldots, x_p, t) = \begin{cases} f\Big((1-t)x_1, x_2, \ldots, x_p\Big) & \text{for } 0 \leq x_1 \leq \frac{1}{2} \\ f\Big((1-t)(1-x_1), x_2, \ldots, x_p\Big) & \text{for } \frac{1}{2} < x_1 \leq 1 \end{cases} \tag{7}$$

(and similarly $[f^{-1}] \circ [f] = [f_\mathfrak{m}]$), meaning that $[f^{-1}] \equiv [f]^{-1}$ is the inverse of $[f]$ under "$\circ$". We have thus made $\pi_p(M, \mathfrak{m})$ with $p \geq 1$ into a group – the *p-th homotopy group of M*.

The homotopy groups have been tabulated for many spaces $M$, including those that appear in the analysis of band-structure nodes, see Ref. [4]. It can be shown that they are Abelian for $p \geq 2$, and that they do not depend on the specific choice of $\mathfrak{m}$ when $M$ is connected [1]. In the latter case, we simplify the notation by writing just $\pi_p(M)$. By identifying $\partial I^p$ as a single point P, one obtains the same group structure also on maps $f : S^p \to M$.

The case $p = 0$ is special, because we lack the direction $x_1$ to define the binary operation in Eq. (2). In other words, if we map the first point of $S^0$ to $\mathfrak{m}$ while the second point lies anywhere in $M$, we cannot define a simple rule for "gluing" two consecutive zero-dimensional spheres together. However, the notion of the equivalence class $[f]$ derived from a map $f$ remains meaningful, as does the collection (i.e. a *set*) of all such equivalence classes. We denote this *homotopy set* as $\pi_0(M)$. In the special cases when $M$ has one (two) *connected components*, the set $\pi_0(M)$ has exactly one (two) elements, and can be perceived as having a $\mathbb{0}$ ($\mathbb{Z}_2$) group structure. More generally, if the connected components of $M$ have a canonical group structure (which is not in general guaranteed) isomorphic to a discrete group $G$, then $\pi_1(M) = G$.

### B. Relative homotopy groups

We now consider continuous maps from a *p-dimensional disc* $D^p$ (i.e. a sphere $S^{p-1}$ with its interior, assuming that $p$ is a *positive integer*) to a topological space $M$, such that the boundary $\partial D^p \cong S^{p-1}$ is mapped to a *subspace* $X \subset M$. Such a scenario with $p = 1$ and $p = 2$ arises when studying the nodes in the presence of $m_z$ or $C_{2z}\mathcal{T}$ symmetry. We show below that the collection of *all* such maps exhibits a group structure for $p \geq 2$ if we make them pointed by pinning a selected point $\mathrm{P} \in \partial D^p$ to a base-point $\mathfrak{m} \in X$, i.e. when

$$f : \begin{array}{rcl} D^p & \to & M \\ \partial D^p & \to & X \\ \partial D^p \supset \mathrm{P} & \to & \mathfrak{m}. \end{array} \tag{8}$$

To simplify the analysis, it is convenient to perform a continuous deformation of $D^p$ into $I^p$ such that the point P is stretched into the entire surface $\partial I^p$ with the exception of the $x_p = 1$ face (also expressible as $I^{p-1} \times \{1\}$). We denote this part of the hypercube surface as

$$J^{p-1} := (\partial I^p) \setminus (I^p \times \{1\}) \tag{9}$$

At the same time, the rest of the cube surface $(\partial D^p)\backslash\{\mathrm{P}\}$ is shrunk to the $x^p = 1$ face. An explicit example of such a deformation for $p = 2$ is shown in Fig. S-1. The originally considered maps on $D^p$ are then transformed into continuous maps fulfilling

$$f: \begin{array}{ccc} I^p & \to & M \\ \partial I^p & \to & X \\ J^{p-1} & \to & \mathfrak{m}. \end{array} \tag{10}$$

Assuming $p \geq 2$, one can define a binary composition (2) that is closed on the set $\widetilde{\pi}_p(M, X, \mathfrak{m})$ of *all* maps fulfilling the conditions (10). However, just like for the case of Sec. II A, the absence of identity element means that $\widetilde{\pi}_p(M, X, \mathfrak{m})$ is only a semigroup.

In analogy with Sec. II A, we instead focus on the set $\pi_p(M, X, \mathfrak{m})$ of *equivalence classes* of maps: Two maps $f_1$ and $f_2$ are equivalent if there exists a homotopy $\mathcal{F} : I^p \times I \to M$ such that $\forall \mathbf{x} \in I^p$ and $\forall t \in I$:

$$\mathcal{F}(\mathbf{x}, 0) = f_1(\mathbf{x}), \qquad \mathcal{F}(\mathbf{x}, 1) = f_2(\mathbf{x}), \qquad \mathcal{F}(\partial I^p, t) \subset X \qquad \text{and} \qquad \mathcal{F}(J^{p-1}, t) = \mathfrak{m}. \tag{11}$$

We write $[f]$ to represent all maps that can be reached from $f$ in this way. Clearly, $[f_1] = [f_2]$ if maps $f_1$ and $f_2$ are equivalent. All the steps from (4) to (7) remain valid, meaning that "$\circ$" makes $\pi_p(M, X, \mathfrak{m})$ into a group – the *p-th relative homotopy group*. The relative homotopy groups $\pi_p(M, X, \mathfrak{m})$ can often be easily found if both $\pi_p(M, \mathfrak{m})$ and $\pi_p(X, \mathfrak{m})$ are already known, as we explicitly show in Sec. II C. It can further be shown that they are Abelian for $p \geq 3$, and that they do not depend on the specific choice of $\mathfrak{m}$ when $X$ is connected. In the latter case we simplify the notation by writing $\pi_p(M, X)$. By identifying $J^{p-1}$ as a single point P, one obtains the same group structure on the original set of maps on $D^p$.

The case $p = 1$ is special, because we lack the direction $x_1$ to define the binary operation in Eq. (2). The problem follows from Eqs. (10) which state that while the lower end $x_p \equiv x_1 = 0$ of the interval $D^1 \equiv I^1$ is mapped to $\mathfrak{m}$, the upper end $x_p \equiv x_1 = 1$ is mapped anywhere in $X$. Therefore, there is no obvious rule for gluing two consecutive intervals into a single one. However, in analogy with the $p = 0$ case of Sec. II A, the notion of the equivalence class $[f]$ of a map $f$ is meaningful, as is the collection (i.e. the *relative homotopy set*) $\pi_1(M, X, \mathfrak{m})$ of all such equivalence classes. One can define a $\mathbb{0}$ ($\mathbb{Z}_2$) group structure on this set if it contains exactly one (two) elements.

### C. Long exact sequence of homotopy classes

Let us consider the following *long sequence* of *homomorphisms* between homotopy groups

$$\ldots \xrightarrow{\partial_{p+1}} \pi_p(X, \mathfrak{m}) \xrightarrow{i_p} \pi_p(M, \mathfrak{m}) \xrightarrow{j_p} \pi_p(M, X, \mathfrak{m}) \xrightarrow{\partial_p} \pi_{p-1}(X, \mathfrak{m}) \xrightarrow{i_{p-1}} \ldots. \tag{12}$$

where:

- $i : X \to M$ is the *inclusion map*, which takes points of $X$ and interprets them as points of $M$. This induces an inclusion $i_p$ of set $\widetilde{\pi}_p(X, \mathfrak{m})$ inside its superset $\widetilde{\pi}_p(M, \mathfrak{m})$. By considering the equivalence classes, this further leads to a homomorphism (if a group structure exists) from $\pi_p(X, \mathfrak{m})$ to $\pi_p(M, \mathfrak{m})$
- $j_p : \pi_p(M, \mathfrak{m} \in X) \to \pi_p(M, X, \mathfrak{m})$ is also an inclusion map, where $f \in \widetilde{\pi}_p(M, \mathrm{m})$ is interpreted as an element of $\widetilde{\pi}_p(M, X, \mathfrak{m})$. Since the latter poses looser boundary condition on the $x_p = 1$ face, obviously $\widetilde{\pi}_p(M, \mathfrak{m}) \subset \widetilde{\pi}_p(M, X, \mathfrak{m})$. By further considering the equivalence classes, we obtain a homomorphism $j_p$ from $\pi_p(M, \mathfrak{m})$ to $\pi_p(M, X, \mathfrak{m})$.
- $\partial_p$ can be understood as a boundary operator. If we stick to the hypercube formulations of homotopy classes via Eqs. (1) and (10), then $\partial_p f$ takes the value of $f \in \widetilde{\pi}_p(M, X, \mathfrak{m})$ on the $x_p = 1$ face, i.e.

  $$(\partial_p f)(x^1, \ldots, x^{p-1}) = f(x^1, \ldots, x^{p-1}, 1). \tag{13}$$

  Alternatively, if one works with the equivalent formulation using discs and spheres, then $\partial_p f$ on $S^{p-1}$ acquires the values of $f$ on $\partial D^p \cong S^{p-1}$.

We show below that sequence (12) is *exact*, meaning that the image of any arrow in the sequence is identical to the kernel of the next one [1]. The exactness provides a convenient computational tool for the relative homotopy classes from the non-relative ones whenever they have a group structure (which may cease to exist once we reach $\pi_1(M, X, \mathfrak{m})$). However, sequence (12) remains exact even when the group structure is lost (i.e. all the way down to the last meaningful set $\pi_0(M, \mathfrak{m})$). Importantly, the arrows in (12) are compatible with the group structure, meaning that they are *homomorphisms*. We can thus take advantage of the relation

$$\operatorname{im} \varphi = G / \ker \varphi \tag{14}$$

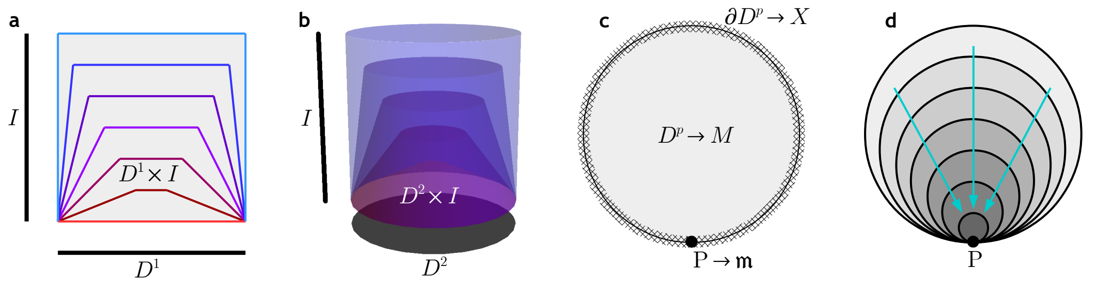


**Figure** S-2. (a) The alternative partitioning of $D^p \times I$ into a family of discs $\widetilde{D}^p$ for $p = 1$ that is used in the proof of the compression criterion. (b) The same partitioning for $p = 2$. The generalization to $p \geq 3$ is straightforward. (c) A schematic representation of a continuous map $f$ on $D^p$ such that $[f] \in \pi_p(M, X, \mathfrak{m})$. The disc $D^p$ (gray) is mapped into $M$, the boundary $\partial D^p \cong S^{p-1}$ (hatched) is mapped into $X$, and the point $\mathrm{P} \in \partial D^p$ (black dot) is mapped onto base-point $\mathfrak{m} \in X$. The boundary operator $\partial_p$ restricts $f$ to the boundary $\partial D^p$, such that the image of $\partial_p f$ lies in $X$. (d) The map $\partial_p f$ is homotopic inside $\pi_{p-1}(M, \mathfrak{m})$ to the constant map if we use $f$ itself as the homotopy. The homotopy can be visualized as a contraction of $S^{p-1} \subset D^p$ onto P as indicated by the blue arrows. Such a homotopy is considered in the proof of $\operatorname{im} \partial_p = \ker i_{p-1}$ of the long sequence (12). Similarly, if we replace in panel (c) the space $M$ by the subspace $X$ and relabel $f$ by $g$, then the analogous panel (d) illustrates the deformation retraction of $g$ onto the constant map as considered in the proof of the compression criterion.

between the image and the kernel of a group homomorphism $\varphi : G \to H$.

Proving the exactness of long sequence (12) requires some work. In the rest of this section, we reproduce and expand the proof appearing in Ref. [1] which assumes the definition of homotopy groups using maps on discs and spheres. An equivalent proof that uses the formulation of homotopy groups using hypercubes appears in Sec. IX.B of Ref. [2].

To proceed, it is convenient to first derive the so-called *compression criterion*, which states that:

> **Compression criterion**: A map $f$ fulfilling (8) is equivalent to the identity element $e$ of $\pi_p(M, X, \mathfrak{m})$ if and only if there exists a continuous homotopy $\widetilde{\mathcal{F}} : D^p \times I \to M$ such that $\forall \mathbf{x} \in D^p$, $\forall \mathbf{y} \in \partial D^p$ and $\forall t \in I$:
>
> $$\widetilde{\mathcal{F}}(\mathbf{x}, 0) = f(\mathbf{x}), \qquad \widetilde{\mathcal{F}}(\mathbf{x}, 1) \in X \qquad \text{and} \qquad \widetilde{\mathcal{F}}(\mathbf{y}, t) = f(\mathbf{y}). \tag{15}$$
>
> This is often expressed briefly by stating that $f$ is *homotopic rel* $\partial D^p$ to a map with image in $X$. By setting $X = \{\mathfrak{m}\}$, conditions (15) reproduce the definition of triviality of $[f] = e$ within $\pi_p(M, \mathfrak{m})$ as given in Sec. II A.

We prove the compression criterion in both directions. First, assume that for a given $f$ there exists a homotopy $\widetilde{\mathcal{F}}$ fulfilling conditions (15). We denote $\widetilde{\mathcal{F}}(\mathbf{x}, 1) \equiv g(\mathbf{x})$, such that the existence of $\widetilde{\mathcal{F}}$ implies $[f] = [g]$ within $\pi_p(M, X, \mathfrak{m})$. But $g(D^p) \subset X$ further implies that $[g] = e$ within $\pi_p(M, X, \mathfrak{m})$. The corresponding homotopy is a retraction of $D^p$ onto point P as illustrated in Fig. S-2(d). We thus conclude that $f$ is equivalent to the identity element $e$ of $\pi_p(M, X, \mathfrak{m})$. To prove the implication in the reverse direction, note that the equivalence $[f] = e$ within $\pi_p(M, X, \mathfrak{m})$ implies the existence of a continuous homotopy $\mathcal{F} : D^p \times I$ such that $\forall \mathbf{x} \in D^p$, $\forall \mathbf{y} \in \partial D^p$ and $\forall t \in I$:

$$\mathcal{F}(\mathbf{x}, 0) = f(\mathbf{x}), \qquad \mathcal{F}(\mathbf{x}, 1) = \mathfrak{m} \qquad \text{and} \qquad \mathcal{F}(\mathbf{y}, t) \in X. \tag{16}$$

Then a homotopy $\widetilde{\mathcal{F}}$ fulfilling Eqs. (15) is obtained by an alternative partitioning of the cylinder $D^p \times I$ into a family of $p$-disks $\widetilde{D}^p$, namely starting with $D^p \times \{0\}$ and ending with $D^p \times \{1\} \cup (\partial D^{p-1}) \times I$. Examples of such a partitioning for $p = 1$ and $p = 2$ are illustrated in Fig. S-2(a,b). All discs $\widetilde{D}^p$ share their boundary at the cost of the last disc being mapped onto $X$ rather than onto the single point $\mathfrak{m}$, as required by Eqs. (15). This completes the proof of the compression criterion.

Let us now prove the exactness of long sequence (12) at the pair $(i_p, j_p)$. A map $f$ such that $[f] \in \operatorname{im} i_p$ is by definition of $i_p$ homotopic rel $\partial D^p$ to a map with image in $X$. On the other hand, a map $f$ such that $[f] \in \ker j_p$ is by definition of $j_p$ equivalent to the identity element $e$ of $\pi_p(M, X, \mathfrak{m})$. By the compression criterion, this is equivalent to $f$ being homotopic rel $\partial D^p$ to a map with image in $X$. Clearly, the sets $\operatorname{im} i_p = \ker j_p$ are equal.

We proceed with proving the exactness of (12) at the pair $(j_p, \partial_p)$. By definition, if $[f] \in \operatorname{im} j_p$, then $f$ is homotopic to a map $\tilde{f}$ such that $\tilde{f}(\partial D^p) = \mathfrak{m}$. But such a map is trivially mapped by $\partial_p$ onto the constant map $[f_\mathfrak{m}] = e$ in $\pi_{p-1}(M, \mathfrak{m})$, hence $\operatorname{im} j_p \subset \ker \partial_p$. Proving the reverse requires a few more steps that are illustrated in Fig. S-3. Let $[f] \in \ker \partial_p$, then by definition $[\partial_p f] = e$ within $\pi_{p-1}(X, \mathfrak{m})$. This implies the existence of a homotopy $\mathcal{F} : D^{p-1} \times I \to X$ such that $\forall \mathbf{x} \in D^{p-1}$, $\forall \mathbf{y} \in \partial D^{p-1}$ and $\forall t \in I$:

$$\mathcal{F}(\mathbf{x}, 0) = (\partial_p f)(\mathbf{x}), \qquad \mathcal{F}(\mathbf{x}, 1) = \mathfrak{m} \qquad \text{and} \qquad \mathcal{F}(\mathbf{y}, t) = \mathfrak{m}. \tag{17}$$

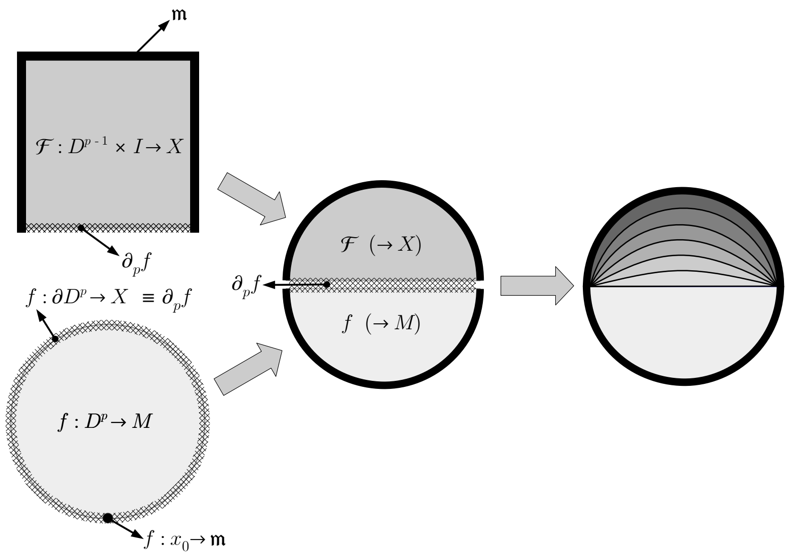


**Figure** S-3. Proving that $\ker \partial_p \subset \operatorname{im} j_p$. We consider a map $f : D^p \to M$ such that $[f] \in \ker \partial_p$, and attempt to glue together the map $f$ and the homotopy $\mathcal{F} : D^{p-1} \times I \to X$ corresponding to the equivalence $[\partial_p f] = e \in \pi_{p-1}(X, \mathfrak{m})$. Hatched boundaries indicate the support of $\partial_p f$, and the thick black lines/points indicate images in $\mathfrak{m}$. To glue the two functions together, we deform both $D^p$ and $D^{p-1} \times I$ into $p$-dimensional semidiscs with the curved part of the boundary taking values in $\mathfrak{m}$ (solid black) and the map $\partial_p f$ being realized on the flat part of the boundary (hatched). We denote the composed "glued" map as $f \oplus \mathcal{F}$. Clearly, $[f \oplus \mathcal{F}] = [f]$ within $\pi_p(M, X, \mathfrak{m})$ using a homotopy that attaches to $f$ increasingly larger "chunks" of $\mathcal{F}$, as indicated in the last panel of the scheme.

We deform the manifold $D^{p-1} \times I$ into a $p$-dimensional semi-disk such that the curved part of the boundary is mapped onto $\mathfrak{m}$ while preserving the map $\partial_p f$ on the flat part of the boundary. Similarly, we deform the original disc $D^p$ with map $f$ into a semidisc, such that point P (mapped by $f$ to $\mathfrak{m}$) is expanded into the curved part of the semidisc boundary, while $D^p \backslash \{\mathrm{P}\}$ deforms into the flat part of the boundary (carrying the map $\partial_p f$). It is then possible to glue the two semidiscs into a complete disc $D^p$ while preserving the continuity of the composed map. We denote the "glued" map on $D^p$ as $f \oplus \mathcal{F}$. Clearly, $f \oplus \mathcal{F}$ maps $\partial D^p$ to $\mathfrak{m}$, therefore $[f \oplus \mathcal{F}] \in \operatorname{im} j_p$. However, $[f \oplus \mathcal{F}] = [f]$ within $\pi_p(M, X, \mathfrak{m})$ using a homotopy that attaches to $f$ an increasingly larger "chunk" of $\mathcal{F}$ as shown in the right part of Fig. S-3. We thus obtain $\ker \partial_p \subset \operatorname{im} j_p$. Collecting both of the subset relations, this paragraph proves that $\operatorname{im} j_p = \ker \partial_p$.

Finally, we tackle the long sequence (12) at pair $(\partial_p, i_{p-1})$. First, let $[f] \in \pi_p(M, X, \mathfrak{m})$ such that $[\partial_p f] \in \operatorname{im} \partial_p$. Then $[i_{p-1} \partial_p f] = e$ within $\pi_{p-1}(M)$ by taking as the homotopy $\mathcal{F} = f$ itself [see Fig. S-2(c,d)], therefore $\operatorname{im} \partial_p \subset \ker i_{p-1}$. To prove the reverse, let $[f] \in \ker i_{p-1}$, such that $[f] = e$ within $\pi_{p-1}(M, \mathfrak{m})$. Therefore, there is a homotopy $\mathcal{F} : D^{p-1} \times I \to M$ such that $\forall \mathbf{x} \in D^{p-1}$, $\forall \mathbf{y} \in \partial D^{p-1}$ and $\forall t \in I$:

$$\mathcal{F}(\mathbf{x}, 0) = f(\mathbf{x}), \qquad \mathcal{F}(\mathbf{x}, 1) = \mathfrak{m} \qquad \text{and} \qquad \mathcal{F}(\mathbf{y}, t) = \mathfrak{m} \tag{18}$$

We can deform $D^{p-1} \times I$ into $D^p$ while contracting $\partial D^{p-1} \times I \cup D^{p-1} \times \{1\}$ to the point P. Then obviously $[\mathcal{F}] \in \pi_p(M, X, \mathfrak{m})$, and the restriction to the surface $\partial D^p$ reproduces $f = \partial_p \mathcal{F}$, therefore $f \in \operatorname{im} \partial_p$. We conclude that $\operatorname{im} \partial_p = \ker i_{p-1}$. Altogether, we proved the exactness of long sequence (12).

We finally list here an additional property of relative homotopy groups which states that [5]

$$X \text{ is null-homotopic inside } M \qquad \Rightarrow \qquad \pi_p(M, X) = \pi_p(M) \times \pi_{p-1}(X) \tag{19}$$

where "×" denotes the *direct product* of two groups, and where *null-homotopic* means to be contractible to a single single point with continuous deformations. If the two groups are Abelian, we replace "×" by "⊕" and call it the *direct sum* [6]. The exactness of sequence (12) together with relations (14) and (19) constitute a powerful set of tools for deriving the relative homotopy groups from the non-relative ones.

## III. ANALYSIS OF BAND-STRUCTURE NODES

In this section, we use the reviewed knowledge of homotopy theory to derive new topological invariants in the presence of mirror or $C_{2z}\mathcal{T}$ symmetry. In Sec. III A, we discuss our strategy in its widest generality. We then follow with an explicit discussion of the systems considered in the main text. In Sec. III B, we consider nodal class A with mirror symmetry, and

determine when a pair of mirror-related WPs cannot annihilate at the symmetric plane, but instead convert into a mirror-protected nodal loop. In Sec. III C, we discuss nodal class A with $C_{2z}\mathcal{T}$ symmetry, when WPs of two-band models carry two independent integer charges. This manifests in non-trivial conversions between in-plane and out-of-plane WPs. Finally, we consider in Sec. III D a superconducting model belonging to nodal class C with $C_{2z}\mathcal{T}$ symmetry. In this case, WPs are again characterized with a pair of integer charges that are manifested by a non-trivial conversion rule. However, as opposed to the semimetallic case, in class C the non-trivial result persists in models with many bands.

### A. General strategy

Stable band-structure nodes and their topological charges can be understood using homotopy theory [3, 7]. The basic idea is to consider a sphere $S^p \subset$ BZ (Brillouin zone), which is automatically equipped with a map (i.e. the Hamiltonian)

$$H : S^p \to M \tag{20}$$

where $M$ is the space of admissible gapped Hamiltonian matrices. If $H$ is also gapped *inside* the $S^p$, then the sphere can be shrunk to a single point without encountering a momentum with gapless spectrum (i.e. a singularity of $H$). Such a contraction continuously deforms $H(S^p)$ into a constant map, i.e. we write $[H] = e$ of some homotopy group. Conversely, if $[H] \neq e$, there must be a singularity of $H$ occurring for at least one momentum $\mathbf{k}_0$ inside $S^p$ which renders such a continuous deformation impossible. The singularity indicates a gapless $H(\mathbf{k}_0)$, i.e. a node inside the $S^p$.

The symmetries of the system enter the discussion at two levels. First, symmetries that are *local* in $\mathbf{k}$-space (i.e. $\mathcal{PT}$, $\mathcal{PC}$ and $\mathcal{CT}$, where $\mathcal{P}$ is spatial inversion, $\mathcal{T}$ is time-reversal, and $\mathcal{C}$ is charge conjugation – these define ten "AZ+$\mathcal{P}$" or "nodal" symmetry classes [3, 8]) constrain the space $M$ of admissible Hamiltonians [9]. This leads one to consider homotopy groups $\pi_p(M)$, which describe nodes occurring at generic low-symmetry momenta inside the Brillouin zone (BZ). Second, symmetries $R$ that are *non-local* in $\mathbf{k}$-space facilitate an additional structure *both* inside the space of Hamiltonians $M$ *and* in the admissible maps $H$. To see these additional structures, note that symmetry $R$ naturally defines symmetric subspaces $\Pi \subset$ BZ in momentum space and $X_R \subset M$ in the space of Hamiltonians through

$$\Pi = \{\mathbf{k} \in \mathrm{BZ} \mid R\mathbf{k} = \mathbf{k}\} \qquad \text{and} \qquad X_R = \left\{H \in M \mid RHR^{-1} = H\right\}, \tag{21}$$

such that $\forall \mathbf{k} \in \Pi : H(\mathbf{k}) \in X_R$. Taking $S^p \subset \Pi$ leads one to consider homotopy groups $\pi_p(X_R)$, which describe nodes lying inside the symmetric subspace $\Pi$. To further reveal the restriction imposed by $R$ on *maps* (20), consider a sphere $S^p$ that is symmetric under $R$ and that has a non-trivial overlap $S^p \cap \Pi \cong S^q$ with $q < p$. Then the map (20) must fulfil a non-local constraint

$$H(R\mathbf{k}) = RH(\mathbf{k})R^{-1}. \tag{22}$$

Especially, if $R$ is a mirror or $C_{2z}\mathcal{T}$ symmetry which map $(k_x, k_y, k_z) \mapsto (k_x, k_y, -k_z)$, then automatically $q = p - 1$. As explained in the main text, such a symmetry-preserving Hamiltonian fulfilling constraint (22) is fully determined by its action on the hemisphere on one side of the $\Pi$ plane. Since a hemisphere is topologically a disc and because the boundary of the disc lies inside the $\Pi$ plane, the equivalence classes of such maps are described by *relative homotopy group* $\pi_p(M, X_R)$.

As demonstrated in the manuscript on examples, $\pi_p(M, X_R)$ determines the conversion rules between the nodes occurring at generic momenta [following from $\pi_p(M)$] and the nodes occurring at $\Pi$ planes [described by $\pi_{p-1}(X_R)$]. Especially, non-trivial conversions occur if there is a sharp subgroup structure $\pi_{p-1}(X_R) < \pi_p(M, X_R)$, i.e. when the complete $R$-symmetric sphere $S^p$ perceives more topological obstructions than its equator $S^q$. Therefore, if we focus on the case $q = p - 1$, the description of band-structure nodes is summarized by the following steps:

1. The local-in-$\mathbf{k}$ symmetries (captured by one of the ten "AZ+$\mathcal{P}$" or "nodal" classes) may facilitate nodes occurring anywhere in BZ. They are described by $\pi_p(M)$ where $M$ is the classifying space of Hamiltonians.

2. Additional symmetry $R$ which is non-local in $\mathbf{k}$-space may facilitate additional species of nodes that are tied to the invariant subspace $\Pi \subset$ BZ. They are described by $\pi_{p-1}(X_R)$ where $X_R$ is the $R$-invariant subspace of $M$ as defined in Eq. (21).

3. The conversion rules between the two species of nodes are described by *relative homotopy* group $\pi_p(M, X_R)$. Non-trivial conversions can occur if $\pi_{p-1}(X_R) < \pi_p(M, X_R)$

For $R \in \{m_z, C_{2z}\mathcal{T}\}$ in three-dimensional systems, which are the primary examples in our work, the invariant subspaces $\Pi$ correspond to the $k_z = 0$ and the $k_z = \pi$ planes of BZ. The homotopy groups that come into play are illustrated in Fig. S-4. The situation $q = p - 2$ which arises e.g. in the presence of rotation symmetry will be studied elsewhere [10]).

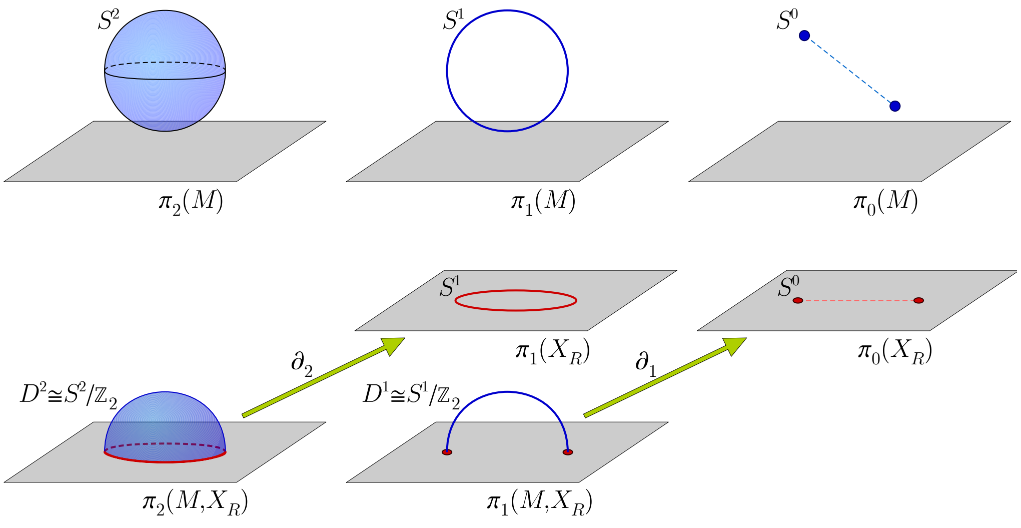


**Figure** S-4. Overview of homotopy groups used to study nodes in the presence of a symmetry $R$ that leads to invariant planes $\Pi$ (grey sheets) in three spatial dimensions. The first row corresponds to generic spheres (blue). They are characterized by homotopy groups $\pi_p(M)$, and describe nodes occurring generically anywhere in the Brillouin zone. If the lowest non-trivial homotopy group corresponds to $p = 2/1/0$, the system exhibits nodal points/lines/surfaces. The second row lists in-plane spheres (red). They are characterized by homotopy groups $\pi_p(X_R)$, and describe nodes tied to the invariant planes. The bottom row indicates spheres that are symmetric under $R$ and that have a non-trivial overlap $S^p \cap \Pi \cong S^{p-1}$ corresponding to the equator (red). Their Hamiltonian maps are fully characterized on a hemisphere $S^p/\mathbb{Z}_2 \cong D^p$ (blue), and their equivalence classes are given by relative homotopy groups $\pi_p(M, X_R)$. Note that the boundary operator $\partial_p$ (green arrows) selects the value of $H$ on the equator. Since the outcome of such a procedure contains less information, there is a subgroup structure $\pi_{p-1}(X_R) \leq \pi_p(M, X_R)$. A sharp inequality can lead to a non-trivial conversion rule between the in-plane and out-of-plane nodes. In the illustration, we order the homotopy groups into columns according to the dimensionality of the considered manifold.

### B. Nodal class A with mirror

A generic two-band Hamiltonian with a spectrum normalized to $\pm 1$ can be uniquely expressed as $H = \mathbf{n} \cdot \boldsymbol{\sigma}$, where $\mathbf{n} \in S^2$ is a unit vector and $\boldsymbol{\sigma} = (\sigma_x, \sigma_y, \sigma_z)$ is a collection of Pauli matrices. In nodal class A [3] there are no additional local-in-$\mathbf{k}$ symmetries that might further constrain the Hamiltonian, therefore $M \cong S^2$. The relevant homotopy groups are

$$\pi_2(M) = \mathbb{Z}, \qquad \pi_1(M) = \mathbb{0} \qquad \text{and} \qquad \pi_0(M) = \mathbb{0}. \tag{23}$$

The lowest non-trivial homotopy group $\pi_2(M) = \mathbb{Z}$ implies that spheres $S^2$ can enclose point-like degeneracies with integer charge. These are Weyl points (WPs) that can occur anywhere in the BZ.

We further assume the presence of a mirror symmetry $m_z : (k_x, k_y, k_z) \mapsto (k_x, k_y, -k_z)$ represented by $\sigma_z$, such that the two orbitals forming the basis of the two-band model have opposite mirror eigenvalues. The space of $m_z$-symmetric Hamiltonians with a normalized spectrum consists of two isolated points, $X_{m_z} = \{+\sigma_z, -\sigma_z\} \cong S^0$. The relevant homotopy groups are

$$\pi_2(X_{m_z}) = \mathbb{0}, \qquad \pi_1(X_{m_z}) = \mathbb{0} \qquad \text{and} \qquad \pi_0(X_{m_z}) = \mathbb{Z}_2. \tag{24}$$

The lowest non-trivial homotopy group $\pi_0(X_{m_z}) = \mathbb{Z}_2$ implies that a pair of points $S^0$ can enclose a robust degeneracy. These degeneracies are nodal lines obtained by crossing of the two bands with opposite mirror eigenvalues. Furthermore, since $\pi_1(X_{m_z}) = \mathbb{0}$ is trivial, any in-plane nodal loop of the two-band model (assuming it does not wind around the BZ torus, such that it can indeed be enclosed by an in-plane $S^1$) can be removed from the symmetric plane. This can be achieved by shrinking the nodal loop to a single point $\mathbf{k}_0 \in \Pi$. (We remark that nodal *loops* imposed by glide planes are unremovable, but require a minimum of four bands and additional time-reversal symmetry [11]!)

We now use the long exact sequence (12) to derive the relative homotopy groups relevant for the description of the nodes. Inserting the known homotopy groups (23) and (24), the sequence becomes

$$\begin{array}{ccccccccccccccccc} \pi_2(X_{m_z}) & \xrightarrow{i_2} & \pi_2(M) & \xrightarrow{j_2} & \pi_2(M, X_{m_z}) & \xrightarrow{\partial_2} & \pi_1(X_{m_z}) & \xrightarrow{i_1} & \pi_1(M) & \xrightarrow{j_1} & \pi_1(M, X_{m_z}) & \xrightarrow{\partial_1} & \pi_0(X_{m_z}) & \xrightarrow{i_0} & \pi_0(M) \\ \mathbb{0} & & \mathbb{Z} & & & & \mathbb{0} & & \mathbb{0} & & & & \mathbb{Z}_2 & & \mathbb{0} \end{array}. \tag{25}$$

It follows from the exactness at $\pi_2(M)$ that $\operatorname{im} i_2 = \mathbb{0} = \ker j_2$. The relation (14) at $j_2$ becomes $\operatorname{im} j_2 = \mathbb{Z}/\mathbb{0} \cong \mathbb{Z}$. By the exactness at $\pi_2(M, X_{m_z})$ also $\ker \partial_2 = \mathbb{Z}$, and for obvious reasons $\operatorname{im} \partial_2 = \mathbb{0}$. Relation (14) at $\partial_2$ reads $\mathbb{0} = \pi_2(M, X_{m_z})/\mathbb{Z}$ which

has a single solution $\pi_2(M, X_{m_z}) = \mathbb{Z}$. To obtain the other result, note that $\ker i_0 = \mathbb{Z}_2$, hence by exactness at $\pi_0(X_{m_z})$ also $\operatorname{im}\partial_1 = \mathbb{Z}_2$. From the other end, obviously $\operatorname{im} j_1 = \mathbb{0} = \ker\partial_2$ where we used exactness at $\pi_1(M, X_{m_z})$. Relation (14) at $\partial_1$ becomes $\mathbb{0} = \pi_1(M, X_{m_z})/\mathbb{Z}_2$, which has a single solution $\pi_1(M, X_{m_z}) = \mathbb{Z}_2$.

Summarizing the previous paragraph, the relative homotopy groups necessary for the description of the nodes are

$$\pi_2(M, X_{m_z}) = \mathbb{Z} \qquad \text{and} \qquad \pi_1(M, X_{m_z}) = \mathbb{Z}_2. \tag{26}$$

Let us discuss the consequences. First, since $\pi_1(M, X_{m_z}) = \pi_0(X_{m_z})$, the semicircle $D^1 \cong S^1/\mathbb{Z}_2$ perceives the same obstructions as its equator $\partial_1 D^1 \cong S^0$. Therefore, this relative homotopy group does not contain any additional information, and describes again the in-plane nodal lines. However, the sharp inequality $\pi_2(M, X_{m_z}) > \pi_1(X_{m_z})$ has non-trivial consequences, manifested by the conversions between pairs of $m_z$-related Weyl points and in-plane ($m_z$-protected) nodal loops. This conversion rule is extensively discussed in the main text, together with the facilitated surfaces states.

Let us turn our attention to the multi-band case. It turns out to be sufficient to consider three-band models. We therefore assume an additional occupied band, and study Hamiltonians with spectrum $\{-1, -1, +1\}$. The space of such Hamiltonians is

$$M \cong \frac{\mathsf{U}(3)}{\mathsf{U}(2) \times \mathsf{U}(1)} = \mathbb{C}P^2 \tag{27}$$

i.e. the complex projective plane [9]. The relevant homotopy groups of this four-dimensional manifold coincide with Eq. (23). To proceed, we represent the mirror operator non-trivially as $m_z = \operatorname{diag}(+1, -1, -1)$, such that a generic $m_z$-symmetric Hamiltonian takes block-diagonal form

$$H = \begin{pmatrix} a & 0 & 0 \\ 0 & \varepsilon + v_z & v_x - \mathrm{i}v_y \\ 0 & v_x + \mathrm{i}v_y & \varepsilon - v_z \end{pmatrix} \qquad \text{with eigenvalues} \qquad \{a, \varepsilon + |\boldsymbol{v}|, \varepsilon - |\boldsymbol{v}|\} \tag{28}$$

where $\boldsymbol{v} = (v_x, v_y, v_z)$ is a real vector, and $a, \varepsilon$ are real scalars. The eigenvector with energy $a$ has positive mirror eignvalue, while the eigenvectors with energy $\varepsilon \pm |\boldsymbol{v}|$ have negative mirror eigenvalue. Therefore, the space $X_{m_z}$ of mirror-symmetric Hamiltonians with normalized spectrum $\{-1, -1, +1\}$ consists of two disconnected pieces

$$X_{m_z} = X_{m_z}^{(-,-)} \cup X_{m_z}^{(+,-)} \tag{29}$$

where the superscript indicates the mirror eigenvalues of the two occupied bands. The component $X_{m_z}^{(-,-)} = \{m_z\}$ consists of a single point (obtained by setting $a = 1$, $\varepsilon = -1$ and $\boldsymbol{v} = \boldsymbol{0}$), while the other component $X_{m_z}^{(+,-)} \simeq S^2$ is homeomorphic to a sphere (obtained by setting $a = -1$, $\varepsilon = 0$ and $|\boldsymbol{v}| = 1$). The zeroth homotopy group $\pi_0(X_{m_z}) = \mathbb{Z}_2$ counts the number of disjoint components of $X_{m_z}$. For the higher homotopy groups we have to be careful about the location of the base point $\mathfrak{m} \in X_{m_z}$, namely

$$\pi_2(X_{m_z}^{(-,-)}) = \mathbb{0}, \qquad \pi_1(X_{m_z}^{(-,-)}) = \mathbb{0}, \tag{30}$$
$$\pi_2(X_{m_z}^{(+,-)}) = \mathbb{Z}, \qquad \pi_1(X_{m_z}^{(+,-)}) = \mathbb{0}. \tag{31}$$

Let us analyze the relative homotopy groups. In both cases, the derivation of $\pi_1(M, X_{m_z})$ is identical to the two-band case, so the result remains $\mathbb{Z}_2$. However, the result for $\pi_2(M, X_{m_z})$ is different when $\mathfrak{m} \in X_{m_z}^{(+,-)}$. In that case, the relevant piece of the long exact sequence is

$$\underset{\mathbb{Z}}{\pi_2(X_{m_z}^{(+,-)})} \xrightarrow{i_2} \underset{\mathbb{Z}}{\pi_2(M)} \xrightarrow{j_2} \pi_2(M, X_{m_z}^{(+,-)}) \xrightarrow{\partial_2} \underset{\mathbb{0}}{\pi_1(X_{m_z}^{(+,-)})} \xrightarrow{i_1} \underset{\mathbb{0}}{\pi_1(M)}. \tag{32}$$

To determine $\pi_2(M, X_{m_z}^{(+,-)})$, we need to obtain additional information about $i_2$. Especially, we need to know what is the $\pi_2(M)$ charge (which is physically the first Chern number) corresponding to the embedding of $S^2 \simeq X_{m_z}^{(+,-)}$ inside $M$. By parametrizing $X_{m_z}^{(+,-)}$ using spherical coordinates $\boldsymbol{v} = (\sin\theta\cos\phi, \sin\theta\sin\phi, \cos\theta)$, it is trivial to check that the embedding carries a non-trivial Chern number $+1$. Therefore, $\operatorname{im} i_2 = \pi_2(M)$ and by exactness of (32) at $\pi_2(M)$ also $\ker j_2 = \pi_2(M)$. Since $j_2$ is a group homomorphism, it follows that $\operatorname{im} j_2 = \mathbb{0}$. By exactness at $\pi_2(M, X_{m_z}^{(+,-)})$ we obtain $\ker\partial_2 = \mathbb{0}$. Obviously, $\operatorname{im}\partial_2 = \mathbb{0}$, so the homomorphism at $\partial_2$ implies trivial $\pi_2(M, X_{m_z}^{(+,-)}) = \mathbb{0}$. Altogether, we find that

$$\pi_2(M, X_{m_z}^{(+,-)}) = \mathbb{0}, \qquad \pi_2(M, X_{m_z}^{(-,-)}) = \mathbb{Z} \qquad \text{and} \qquad \pi_1(M, X_{m_z}) = \mathbb{Z}_2. \tag{33}$$

We thus conclude that the non-trivial conversion rule is lost when the two occupied bands at the equator have opposite $m_z$ eigenvalues.

Our conclusion generalizes to systems with more bands. Basically, if at least two occupied (or two unoccupied) bands have opposite mirror eigenvalue, the corresponding component of the space $X_{m_z}$ has become large enough to unwind any non-trivial

winding of $D^2$ in $M$, such that a pair of $m_z$-related Weyl points can mutually annihilate at the $\Pi$ plane. In Sec. VI we show that the conversion rules can survive in a weaker form *provided that* the additional degrees of freedom are only weakly coupled to the original two bands. On the other hand, if all the occupied bands at the equator have the same eigenvalue (which is assumed to be the opposite of the mirror eigenvalue of all the unoccupied bands), then the non-trivial conversion rule persists in the original form even in the multi-band case. This is because under such circumstances the corresponding component of $X_{m_z}$ is point-like and has a trivial second homotopy group. Such a scenario possibly describes the conversion of nodes observed in the Luttinger model in applied magnetic field, as reported in Ref. [12].

### C. Nodal class A with $C_{2z}\mathcal{T}$

We consider again a two-band model belonging to nodal class A, such that $M = S^2$ with the homotopy groups listed in Eq. (23). The generic nodes occurring outside the symmetric plane $\Pi$ are WPs with integer charge. We now include antiunitary symmetry $C_{2z}\mathcal{T}$ squaring to $+\mathbf{1}$, which we represent by the complex conjugation $K$. We remark that a different representation has been adopted in the main text for illustration purposes, but this does not affect any of the conclusions. In the chosen representation, the space of $C_{2z}\mathcal{T}$-symmetric Hamiltonians is spanned by $\sigma_x$ and $\sigma_z$, such that $X_{C_{2z}\mathcal{T}} \cong S^1$. The relevant homotopy groups are

$$\pi_2(X_{C_{2z}\mathcal{T}}) = \mathbb{0}, \qquad \pi_1(X_{C_{2z}\mathcal{T}}) = \mathbb{Z} \qquad \text{and} \qquad \pi_0(X_{C_{2z}\mathcal{T}}) = \mathbb{0}. \tag{34}$$

Therefore, the generic nodes occurring inside the invariant plane are points characterized by an integer winding number which we call *helicity* in the main text. These are WPs locked to the symmetric plane by $C_{2z}\mathcal{T}$ [13]. At this stage of the discussion it is not clear whether the chirality and the helicity of a given WP are independent or related quantities.

We now determine the relative homotopy groups. Plugging results (23) and (34) into the long sequence (12), we obtain

$$\underset{\mathbb{0}}{\pi_2(X_{C_{2z}\mathcal{T}})} \xrightarrow{i_2} \underset{\mathbb{Z}}{\pi_2(M)} \xrightarrow{j_2} \pi_2(M, X_{C_{2z}\mathcal{T}}) \xrightarrow{\partial_2} \underset{\mathbb{Z}}{\pi_1(X_{C_{2z}\mathcal{T}})} \xrightarrow{i_1} \underset{\mathbb{0}}{\pi_1(M)} \xrightarrow{j_1} \pi_1(M, X_{C_{2z}\mathcal{T}}) \xrightarrow{\partial_1} \underset{\mathbb{0}}{\pi_0(X_{C_{2z}\mathcal{T}})} \xrightarrow{i_0} \underset{\mathbb{0}}{\pi_0(M)}. \tag{35}$$

Since $X_{C_{2z}\mathcal{T}} \cong S^1$ is clearly *null-homotopic* inside $M \cong S^2$, it follows from (19) that

$$\pi_2(M, X_{C_{2z}\mathcal{T}}) = \mathbb{Z} \oplus \mathbb{Z} \qquad \text{and} \qquad \pi_1(M, X_{C_{2z}\mathcal{T}}) = \mathbb{0}. \tag{36}$$

Since $\pi_2(M, X_{C_{2z}\mathcal{T}}) > \pi_1(X_{C_{2z}\mathcal{T}})$, a non-trivial conversion rule exist between the in-plane and the out-of-plane WPs. Especially, the helicity and the chirality of WPs are indeed *independent* topological charges. Also trivially, the helicity of out-of-plane WPs is zero. The details of the conversion rules and the implications for the surface states following from this additional integer invariant are discussed in the main text of the manuscript.

Let us see what changes in a multi-band scenario. We assume an additional occupied band, such that the space of Hamiltonians with normalized spectrum becomes (27) with homotopy groups (23). If we represent $C_{2z}\mathcal{T}$ by $K$, then the space of $C_{2z}\mathcal{T}$-symmetric Hamiltonians corresponds to the *real subspace* of (27), which is the *real* projective plane

$$X_{C_{2z}\mathcal{T}} \cong \frac{\mathsf{O}(3)}{\mathsf{O}(2) \times \mathsf{O}(1)} = \mathbb{R}P^2 \tag{37}$$

with homotopy groups

$$\pi_2(X_{C_{2z}\mathcal{T}}) = \mathbb{Z}, \qquad \pi_1(X_{C_{2z}\mathcal{T}}) = \mathbb{Z}_2 \qquad \text{and} \qquad \pi_0(X_{C_{2z}\mathcal{T}}) = \mathbb{0}. \tag{38}$$

This is a two-dimensional manifold. The reality of (37) implies that the first Chern number of the embedding of $X_{C_{2z}\mathcal{T}}$ inside $M$ [corresponding to $\pi_2(M)$] is trivial. Therefore, $X_{C_{2z}\mathcal{T}}$ is null-homotopic inside $M$, such that statement (19) implies

$$\pi_2(M, X_{C_{2z}\mathcal{T}}) = \mathbb{Z} \oplus \mathbb{Z}_2 \qquad \text{and} \qquad \pi_1(M, X_{C_{2z}\mathcal{T}}) = \mathbb{0}.. \tag{39}$$

It follows that any pair of in-plane WPs can be either moved outside the symmetric plane (if they have the same chirality) or mutually annihilated (if they have opposite chirality). This is a considerable simplification compared to the two-band model discussed previously. It is staightfoward to show that result (39) persists if we keep including additional bands.

### D. Nodal class C with $C_{2z}\mathcal{T}$

As the final example, we discuss a situation where a non-trivial conversion rule survives in the stable limit of many bands. The example is relevant for centrosymmetric systems that develop an even-parity superconducting order parameter breaking

both $\mathcal{T}$ and $C_{2z}$, while preserving the composition $C_{2z}\mathcal{T}$. The system is further assumed to preserve the SU(2) symmetry in the spin degree of freedom. Similar superconducting orders have been very recently analysed in Ref. [8]. Below, we derive the space of Hamiltonians $M$ for generic momenta $\mathbf{k} \in$ BZ, and the subspace $X_{C_{2z}\mathcal{T}} \subset M$ of $C_{2z}\mathcal{T}$-symmetric Hamiltonians for momenta lying in the $k_z = 0$ and $k_z = \pi$ planes. With this knowledge, we further analyse the relevant homotopy groups. Our notation largely follows that of Ref. [3].

The most general Bogolyubov-de Gennes (BdG) Hamiltonian in the absence of symmetries is [14]

$$H(\mathbf{k}) = \begin{pmatrix} \Xi_{\mathbf{k},\uparrow\uparrow} & \Xi_{\mathbf{k},\uparrow\downarrow} & \Delta_{\mathbf{k},\uparrow\uparrow} & \Delta_{\mathbf{k},\uparrow\downarrow} \\ \Xi^\dagger_{\mathbf{k},\uparrow\downarrow} & \Xi_{\mathbf{k},\downarrow\downarrow} & \Delta_{\mathbf{k},\downarrow\uparrow} & \Delta_{\mathbf{k},\downarrow\downarrow} \\ -\Delta^*_{-\mathbf{k},\uparrow\uparrow} & -\Delta^*_{-\mathbf{k},\uparrow\downarrow} & -\Xi^\top_{-\mathbf{k},\uparrow\uparrow} & -\Xi^*_{-\mathbf{k},\uparrow\downarrow} \\ -\Delta^*_{-\mathbf{k},\downarrow\uparrow} & -\Delta^*_{-\mathbf{k},\downarrow\downarrow} & -\Xi^\top_{-\mathbf{k},\uparrow\downarrow} & -\Xi^\top_{-\mathbf{k},\downarrow\downarrow} \end{pmatrix} \equiv \begin{pmatrix} \Xi_{\mathbf{k}} & \Delta_{\mathbf{k}} \\ -\Delta^*_{-\mathbf{k}} & -\Xi^\top_{-\mathbf{k}} \end{pmatrix} \tag{40}$$

where $\Xi_{\mathbf{k}}$ corresponds to the Hamiltonian of the normal state, and $\Delta_{\mathbf{k}}$ is the gap function. The spin components $\Xi_{\mathbf{k},\alpha\beta}$ and $\Delta_{\mathbf{k},\alpha\beta}$ could still contain additional orbital degree of freedom. The Hermiticity and the fermionic statistics require that

$$\Xi_{\mathbf{k}} = \Xi^\dagger_{\mathbf{k}} \qquad \text{and} \qquad \Delta_{\mathbf{k}} = -\Delta^\top_{-\mathbf{k}}. \tag{41}$$

At the level of spin components, these conditions imply that $\Xi_{\mathbf{k},\uparrow\uparrow}$ and $\Xi_{\mathbf{k},\downarrow\downarrow}$ are Hermitian. All additional constraints following from Eqs. (41) are already implemented in the expression (40). Note that the Hamiltonian (40) is automatically equipped with charge-conjugation symmetry

$$\mathcal{C}_t = s_x K, \qquad \mathcal{C}_t^2 = +\mathbf{1}, \qquad \mathcal{C}_t H(\mathbf{k}) \mathcal{C}_t^{-1} = -H(-\mathbf{k}) \tag{42}$$

where Pauli matrices "$s_i$" correspond to the particle-hole degree of freedom, and $K$ is the complex conjugation.

We want the superconducting state to preserve the SU(2) spin-rotation symmetry. From the practical perspective, this indicates the absence of spin-orbit coupling as well as a purely singlet pairing of the electrons. The spin-rotation symmetry is achieved by requiring the BdG Hamiltonian (40) to commute with the generators of spin rotations $J_i = \mathrm{diag}\left(\sigma_i, -\sigma_i^\top\right)$ for $i = 1, 2, 3$ [15] where Pauli matrices "$\sigma_i$" corresponds to the spin degree of freedom. Commutation with $J_z$ leads to

$$\Xi_{\mathbf{k},\uparrow\downarrow} = 0 \qquad \text{and} \qquad \Delta_{k,\uparrow\uparrow} = 0 = \Delta_{k,\downarrow\downarrow}. \tag{43}$$

Commutation with $J_x$ leads to a further constraints

$$\Xi_{\mathbf{k},\uparrow\uparrow} = \Xi_{\mathbf{k},\downarrow\downarrow} \qquad \text{and} \qquad \Delta_{k,\downarrow\uparrow} = -\Delta_{k,\uparrow\downarrow}. \tag{44}$$

Since $J_y = \mathrm{i} J_x J_z$, the third commutation relation is automatically fulfilled. The most general SU(2)-symmetric BdG Hamiltonian thus takes the form

$$H(\mathbf{k}) = \begin{pmatrix} \Xi_{\mathbf{k},\uparrow\uparrow} & 0 & 0 & \Delta_{\mathbf{k},\uparrow\downarrow} \\ 0 & \Xi_{\mathbf{k},\uparrow\uparrow} & -\Delta_{\mathbf{k},\uparrow\downarrow} & 0 \\ 0 & -\Delta^*_{-\mathbf{k},\uparrow\downarrow} & -\Xi^\top_{-\mathbf{k},\uparrow\uparrow} & 0 \\ \Delta^*_{-\mathbf{k},\uparrow\downarrow} & 0 & 0 & -\Xi^\top_{-\mathbf{k},\uparrow\uparrow} \end{pmatrix} \tag{45}$$

We observe that a block-structure has appeared. The 2×2 block in the center

$$H_{\mathrm{red.}} = \begin{pmatrix} \Xi_{\mathbf{k},\uparrow\uparrow} & -\Delta_{\mathbf{k},\uparrow\downarrow} \\ -\Delta^*_{-\mathbf{k},\uparrow\downarrow} & -\Xi^\top_{-\mathbf{k},\uparrow\uparrow} \end{pmatrix} \tag{46}$$

is related by charge-conjugation symmetry (42) to the other block. This implies that all the information about the Hamiltonian is already contained in the block (46), while the other block is redundant. We refer to the block in Eq. (46) as the *reduced BdG* Hamiltonian. It has lost symmetry (42), but it exhibits a *new* charge-conjugation symmetry [15]

$$\mathcal{C}_s = \mathrm{i}\zeta_y K, \qquad \mathcal{C}_s^2 = -\mathbf{1}, \qquad \mathcal{C}_s H_{\mathrm{red.}}(\mathbf{k}) \mathcal{C}_s^{-1} = -H_{\mathrm{red.}}(-\mathbf{k}) \tag{47}$$

where Pauli matrices "$\zeta_i$" correspond to the two-level degree of freedom explicitly shown in Eq. (46) [3]. The presence of $\mathcal{C}_s$ locates SU(2)-symmetric superconductors without additional symmetries in *Altland-Zirnbauer* class C [15].

We further assume the presence of spatial inversion $\mathcal{P}$. Its action is trivial in the spin degree of freedom, and diagonal (i.e. $\mathbf{1}_s$ or $s_z$) in the particle-hole degree of freedom. If we denote the action of spatial inversion in the orbital degree of freedom as $\mathcal{P}_0$ (which is real and fulfils $\mathcal{P}_0^2 = \mathbf{1}$), the representation in the reduced BdG picture of Eq. (46) becomes $\mathcal{P} = \mathrm{diag}\,(\mathcal{P}_0, \pm\mathcal{P}_0)$. Requiring that $\mathcal{P} H_{\mathrm{red.}}(\mathbf{k}) \mathcal{P}^{-1} = H_{\mathrm{red.}}(-\mathbf{k})$ leads to

$$\Xi_{-\mathbf{k},\uparrow\uparrow} = \mathcal{P}_0 \Xi_{\mathbf{k},\uparrow\uparrow} \mathcal{P}_0 \qquad \text{and} \qquad \pm\,\mathcal{P}_0 \Delta_{\mathbf{k},\uparrow\downarrow} \mathcal{P}_0 = -\Delta_{-\mathbf{k},\uparrow\downarrow} \quad = \Delta_{\mathbf{k},\downarrow\uparrow} = \Delta_{\mathbf{k},\uparrow\downarrow} \tag{48}$$

where in the last two steps we used properties (41) and (44) following from the fermionic statistics and from the SU(2) spin-rotation symmetry. The minus sign in Eq. (48) is only possible in multiband superconductors with purely inter-band pairing and vanishing intra-band pairing [3]. This is highly fine-tuned and a very artificial situation, so we instead focus on the positive sign, i.e. *even parity* singlet superconductors with $\mathcal{P} = \mathcal{P}_0 \otimes \mathbf{1}_\zeta$. Since $[\mathcal{P}, \mathcal{C}_s] = 0$ commute, the reduced BdG Hamiltonian exhibits a local-in-$\mathbf{k}$ symmetry

$$\mathcal{P}\mathcal{C}_s = \mathrm{i}\mathcal{P}_0 \otimes \zeta_y K, \qquad (\mathcal{P}\mathcal{C}_s)^2 = -\mathbf{1}, \qquad (\mathcal{P}\mathcal{C}_s) H_{\mathrm{red.}}(\mathbf{k}) (\mathcal{P}\mathcal{C}_s)^{-1} = -H_{\mathrm{red.}}(\mathbf{k}). \tag{49}$$

Due to the absence of time-reversal symmetry, no additional local-in-$\mathbf{k}$ symmetries are present. Therefore, condition (49) locates even-parity superconductors with SU(2) spin-rotation symmetry in *nodal* class C. The corresponding space of Hamiltonians with normalized spectrum is $M \cong M_{\mathrm{C}} = \mathsf{Sp}(n)/\mathsf{U}(n)$ [3] where $n$ is the number of involved orbitals. The homotopy groups

$$\pi_2(M) = \mathbb{Z}, \qquad \pi_1(M) = \mathbb{0} \qquad \text{and} \qquad \pi_0(M) = \mathbb{0} \tag{50}$$

imply the possibility of WPs with integer charge occuring at a generic $\mathbf{k} \in \mathrm{BZ}$.

Let us further consider the presence of $C_{2z}\mathcal{T}$ symmetry. The time-reversal symmetry $\mathcal{T}$ acts in the BdG space as $\mathrm{i}\sigma_y \otimes \mathbf{1}_s K$ [15]. The $\pi$-rotation around the $z$-axis $C_{2z}$ corresponds to a permutation of the orbitals by $R_0$ (which is real and fulfills $R_0^2 = \mathbf{1}$) composed with a rotation $\exp[\mathrm{i}\frac{\pi}{2}\sigma_z] = \mathrm{i}\sigma_z$ in the spin degree of freedom. Finally, the rotation operator has to be diagonal in the particle-hole degree of freedom, i.e. proportional to $\mathbf{1}_s$ or $s_z$. Collecting all three contributions, we find that the representation of the two-fold rotation symmetry in the BdG space is $C_{2z} = \mathrm{i}\,\mathrm{diag}\,(R_0, -R_0, \pm R_0, \mp R_0)$. The composition with time-reversal thus takes the form

$$C_{2z}\mathcal{T} = \mathrm{i}\begin{pmatrix} 0 & R_0 & 0 & 0 \\ R_0 & 0 & 0 & 0 \\ 0 & 0 & 0 & \pm R_0 \\ 0 & 0 & \pm R_0 & 0 \end{pmatrix} K \tag{51}$$

which squares to $+\mathbf{1}$, as expected. Commutation of operator (51) with the BdG Hamiltonian (45) implies

$$\Xi_{C_{2z}\mathbf{k},\uparrow\uparrow} = R_0 \Xi^{\top}_{\mathbf{k},\uparrow\uparrow} R_0 \qquad \text{and} \qquad \Delta_{C_{2z}\mathbf{k},\uparrow\downarrow} = \mp R_0 \Delta^{*}_{\mathbf{k},\uparrow\downarrow} R_0. \tag{52}$$

Inserting these constraints into the reduced BdG Hamiltonian (46) reveals that it is symmetric under $C_{2z}\mathcal{T} = \mathrm{diag}(R_0, \mp R_0)$. This is an antiunitary symmetry that fulfils

$$(C_{2z}\mathcal{T})^2 = +\mathbf{1} \qquad \text{and} \qquad (C_{2z}\mathcal{T}) H(\mathbf{k}_\parallel) (C_{2z}\mathcal{T})^{-1} = H(\mathbf{k}_\parallel) \tag{53}$$

for all momenta $\mathbf{k}_\parallel$ lying inside the $k_z = 0$ and $k_z = \pi$ planes. In combination with symmetry (49), condition (53) implies that the reduced BdG Hamiltonians inside $C_{2z}\mathcal{T}$-invariant planes belongs to nodal class CI. The space of such Hamiltonians is $X_{C_{2z}\mathcal{T}} \cong M_{\mathrm{CI}} = \mathsf{U}(n)/\mathsf{O}(n)$ [3] with homotopy groups

$$\pi_2(M_{C_{2z}\mathcal{T}}) = \mathbb{Z}_2, \qquad \pi_1(M_{C_{2z}\mathcal{T}}) = \mathbb{Z} \qquad \text{and} \qquad \pi_0(M_{C_{2z}\mathcal{T}}) = \mathbb{0}. \tag{54}$$

The non-trivial first homotopy group facilitates WPs locked inside the high-symmetry planes by the $C_{2z}\mathcal{T}$ symmetry, similar to the semimetallic case discussed in Sec. III C. However, while the helicity of Weyl points in the semimetallic class A model was only $\mathbb{Z}_2$-valued in the presence of multiple bands, we show below that the integer character of helicity in the superconducting class C is *unaffected* by the additional bands.

To determine the relative homotopy groups $\pi_p(M, X_{C_{2z}\mathcal{T}})$, we consider the long exact sequence (12) and plug in the known homotopy groups (50) and (54). We obtain

$$\underset{\mathbb{Z}_2}{\pi_2(X_{C_{2z}\mathcal{T}})} \xrightarrow{i_2} \underset{\mathbb{Z}}{\pi_2(M)} \xrightarrow{j_2} \pi_2(M, X_{C_{2z}\mathcal{T}}) \xrightarrow{\partial_2} \underset{\mathbb{Z}}{\pi_1(X_{C_{2z}\mathcal{T}})} \xrightarrow{i_1} \underset{\mathbb{0}}{\pi_1(M)} \xrightarrow{j_1} \pi_1(M, X_{C_{2z}\mathcal{T}}) \xrightarrow{\partial_1} \underset{\mathbb{0}}{\pi_0(X_{C_{2z}\mathcal{T}})} \xrightarrow{i_0} \underset{\mathbb{0}}{\pi_0(M)}. \tag{55}$$

It is not clear whether $X_{C_{2z}\mathcal{T}}$ is null-homotopic inside $M$, so we take the long route. First, the only solution for $\pi_1(M, C_{C_{2z}\mathcal{T}})$ is clearly $\mathbb{0}$. For the second relative homotopy group, note that $\mathrm{im}\, i_2 = \mathbb{0}$, because the monopole charge $\pi_2(X_{C_{2z}\mathcal{T}})$ corresponds to a trivial Chern number $\pi_2(M)$ [3]. It follows that $\ker j_2 = \mathbb{Z}$ and $\mathrm{im}\,\partial_2 = \mathbb{Z}$. It can be shown that there are only two solution for $\pi_2(M_{C_{2z}\mathcal{T}})$, namely the Abelian direct sum $\mathbb{Z} \oplus \mathbb{Z}$ and the non-Abelian semi-direct product $\mathbb{Z} \rtimes \mathbb{Z}$ with binary composition $(a, b) \circ (c, d) = \left(a + (-1)^b c, b + d\right)$ [16]. However, it is obvious that one integer corresponds to the *chirality* and the other to the *helicity* of the WPs enclosed by the $C_{2z}\mathcal{T}$-symmetric sphere. Both topological invariants are manifestly additive under gluing two adjacent hemispheres, therefore

$$\pi_2(M, X_{C_{2z}\mathcal{T}}) = \mathbb{Z} \oplus \mathbb{Z} \qquad \text{and} \qquad \pi_1(M, X_{C_{2z}\mathcal{T}}) = \mathbb{0}. \tag{56}$$

Similar to the case of the two-band semimetallic model of Sec. III C, the non-trivial $\pi_2(M, X_{C_{2z}\mathcal{T}}) > \pi_1(X_{C_{2z}\mathcal{T}})$ implies a non-trivial conversion rule between the in-plane and out-of-plane WPs. Even in the presence of many bands, any process involving a conversion or annihilation of a collection of WPs has to preserve *both* integer invariants.

## IV. LATTICE MODELS

This section introduces the two-band semimetallic lattice Hamiltonians considered in the main text of our work. In Sec. IV A, we present a mirror-symmetric Hamiltonian that exhibits a conversion of $m_z$-related WPs into an $m_z$-protected nodal loop upon varying the model parameters. The resulting nodal-line (NL) phase exhibits both Fermi arcs and drumhead states on its surface. We comment on the chirality and on the stability of the observed Fermi arcs. In Sec. IV B, we introduce a Hamiltonian that preserves two non-trivially represented mirror symmetries. By tuning the model parameters, we can reach either a nodal-line semimetal (NLSM) or a nodal-chain semimetal phase, both exhibiting multiple surface Fermi arcs. The symmetry further admits the possibility to convert a nodal chain into quadruple Weyl points. Finally, in Sec. IV C we introduce a model Hamiltonian with $C_{2z}\mathcal{T}$ symmetry, and demonstrate the non-trivial conversion between in-plane and out-of-plane WPs.

### A. Lattice model for the topologically non-trivial nodal loop on a mirror invariant plane

The considered two-band Hamiltonian for the topologically non-trivial NLSM with a mirror symmetry is

$$H(\mathbf{k}) = D\sin k_z\left(\sin k_x\sigma_x + \sin k_y\sigma_y\right) + \left(A - B\cos k_x - B\cos k_y - C\cos k_z\right)\sigma_z \tag{57}$$

where $A, B, C, D$ are tunable band parameters. The mirror symmetry $m_z$ is represented by $\sigma_z$, such that the system satisfies $\sigma_z H(k_x, k_y, k_z)\sigma_z = H(k_x, k_y, -k_z)$. There are two mirror invariant planes in the Brillouin zone, located at $k_z = 0$ and $k_z = \pi$, respectively. We set

$$A = 1, \qquad B = 0.8 \qquad \text{and} \qquad D = 1, \tag{58}$$

and treat $C$ as a free parameter.

We first discuss the case $C = 0$. The Hamiltonian on the mirror-invariant planes $k_z = 0$ and $k_z = \pi$ is given by

$$H(k_x, k_y, 0 \text{ or } \pi) = (A - B\cos k_x - B\cos k_y)\sigma_z. \tag{59}$$

Note that the Hamiltonian does not change under flipping the sign of $k_x$ or $k_y$. For parameters (58), the gapless points form two NLs centred at $k_x = k_y = 0$, i.e. one in each invariant plane. We can check that both NLs are associated with a non-trivial winding number $n_\mathrm{W} \in \pi_2(M, X_{m_z})$. To demonstrate that this is indeed the case, we expand the Hamiltonian near $k_x = k_y = k_z = 0$ to quadratic order, such that approximately

$$H_{\text{eff.}}(\mathbf{k}) = Dk_zk_x\sigma_x + Dk_zk_y\sigma_y + \left[A - 2B + \tfrac{1}{2}(k_x^2 + k_y^2)\right]\sigma_z \equiv \mathbf{d}(\mathbf{k}) \cdot \boldsymbol{\sigma} \tag{60}$$

which produces a circular NL at $k_z = 0$ with radius $r_\mathrm{NL} = (4B - 2A)^{1/2}$. We enclose the NL with a sphere of radius $R > r_\mathrm{NL}$ and take advantage of spherical coordinates

$$k_x = R\sin\theta\cos\phi, \quad k_y = R\sin\theta\sin\phi \quad \text{and} \quad k_z = R\cos\theta. \tag{61}$$

We can compute the winding number by adjusting the parameters to more convenient values $2B - A = 1/4, D = 1/2$ and $R = 1$, which slightly shrinks the NL without changing the winding number. Then the $\mathbf{d}(\mathbf{k})$ on the sphere becomes simple, $\mathbf{d} = \frac{1}{4}(\sin 2\theta\cos\phi, \sin 2\theta\sin\phi, -\cos 2\theta)$, and an explicit integration leads to

$$n_\mathrm{W} = \frac{1}{4\pi}\int_0^{\pi/2} d\theta \int_0^{2\pi} d\phi \frac{\mathbf{d}\cdot(\partial_\theta\mathbf{d} \times \partial_\phi\mathbf{d})}{|\mathbf{d}|^3} = -1. \tag{62}$$

As $C$ is increased to positive values, the gapless momenta in the $k_z = 0$ ($k_z = \pi$) plane satisfy

$$A - B\cos k_x - B\cos k_y = +C \ \ (-C), \tag{63}$$

such that the NL expands (shrinks). The corresponding Hamiltonian at the $k_z = 0$ and $\pi$ planes remains symmetric under flipping the sign of $k_x$ or $k_y$. The value $C = 0.3$ corresponds to surface spectra plotted in Fig. 2(a-b) of the main text. As $C$ is increased above the critical value $C_\text{crit.} = 0.6$ , the NL at $k_z = \pi$ shrinks to a single point and subsequently converts into a pair of $m_z$-related WPs. We plot the surface spectra for C = 0.9 on the other side of the topological phase transition in Fig. 2(c-d) of the main text.

We observed in Fig. 2(a,c) of the main text, that $m_z$-protected nodal loops carrying a non-trivial value of $n_\mathrm{W}$ are connected by a pair of surface Fermi arcs to projections of other nodes in the (100) surface BZ. These Fermi arcs are chiral, as shown for a cut along $k_y$-axis at fixed $k_z = -\pi/2$ in Fig. S-5(a). The presence of the chiral Fermi arcs follows from bulk-boundary correspondence, and the argument is analogous to that for Weyl points [17]: Consider a smooth interpolation between the

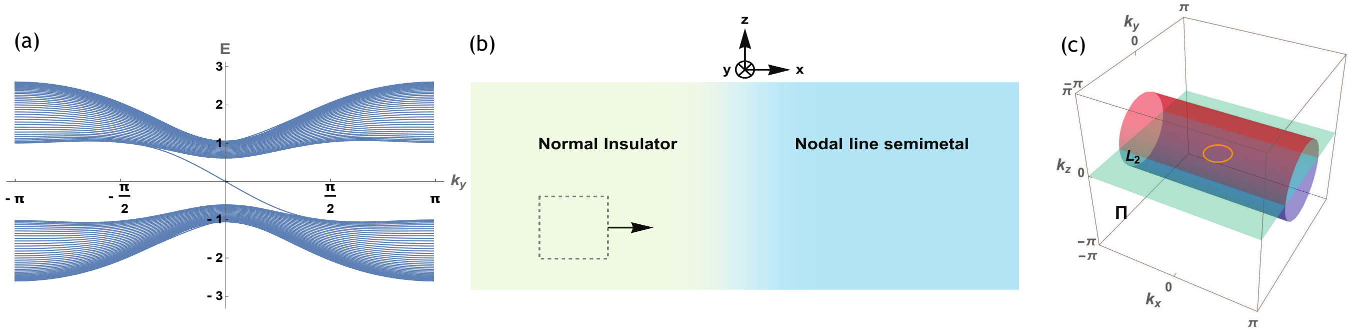


**Figure** S-5. (a) Surface states obtained for the Hamiltonian in Eq. (57) for open boundary condition in the (100) direction. We set $A = 1$, $B = 0.8$, $C = 0.3$ and $D = 1$, corresponding to Fig. 2(a-b) of the main text, and we study the spectrum on the front surface along a cut in the $k_y$-direction for fixed $k_z = -\pi/2$. We took $N = 40$ layers in the numerical calculations. The observed Fermi arc is clearly chiral. (b) The appearance of the pair of Fermi arcs in Fig. 2(a,c) of the main text can be understood through bulk-boundary correspondence. Let us consider a smooth interpolation between a normal insulator (NI, beige) and NLSM (blue), such that any small region (moving dashed square) can be treated as having an approximate translational invariance. (c) Since the (100) surface is symmetric under $m_z$ symmetry, every such a small region has a well-defined second relative homotopy invariant (26) on a half-torus projecting onto a semicircle in the $k_y, k_z$-plane. Since the invariant on the half-torus takes different values for the NI and the NLSM phase, a gap closing has to occur on the semicircle at the interface, leading to the appearance of surface Fermi arcs.

Hamiltonian of a normal insulator (NI) on one side and a NLSM phase on the other side of a (100) boundary [Fig. S-5(b)]. Then we can take a small region moving in the $x$-direction and treat it as having an approximate translational invariance, leading to a proper three-dimensional BZ. Since the (100) boundary preserves $m_z$ symmetry which facilitates the second relative homotopy invariant in Eq. (26), we can assign each such a small region the appropriate value of this invariant on a (semi)cylinder in BZ that encloses the nodal-loop of the NLSM phase. Since this invariant changes from $n_{\mathrm{W}} = 0$ for NI to $n_{\mathrm{W}} = \pm 1$ for NLSM, a gap closing has to occur on each semi-cylinder somewhere on the interface. This implies the presence of an $m_z$-related pair of surface Fermi arcs crossing the circular projection of the bulk cylinder, in agreement with our observations in Fig. 2(a,c) of the main text.

The discussed surface Fermi arcs are chiral, and therefore cannot open a gap through hybridization (excluding particle-hole channel in superconductors, and finite-momentum scattering which breaks the translational invariance [18, 19]). Continuous $m_z$-symmetric perturbations of the bulk Hamiltonian or of the boundary condition lead to a continuous motion of the Fermi arcs in the surface BZ. Since the Hamiltonians corresponding to Eqs. (59) and (63) are symmetric in $k_y$, the 1D edges of the semi-cylinders in Fig. S-5 have identical spectra. Identifying them allows us to interpret the semi-cylinders as closed manifolds, such that each semi-cylinder has to support $|n_{\mathrm{W}}|$ Fermi arcs. Removing the accidental symmetry forbids us to treat the semi-cylinders as closed manifolds, and allows one to detach the surface Fermi arcs from the projections of the bulk nodal loops. However, we observe that such a detachment requires a finite amount of perturbation, and does not occur for weak perturbations.

### B. Lattice model for the topologically non-trivial nodal-chain in the presence of two mirror symmetries

The considered two-band model Hamiltonian for the topologically non-trivial nodal-chain semimetal is

$$\begin{aligned} H(\mathbf{k}) = &\Big[A + B_1(\cos 2k_x + \cos 2k_y) - B_2(\cos k_x - \cos k_y) - C\cos k_x \cos k_y - D\cos k_z\Big]\sigma_z \\ &+ E\Big(\sin 2k_x \sin 2k_y + \sin k_x \sin k_y\Big)\sigma_x + E\sin k_x \sin k_y \sin k_z \sigma_y, \end{aligned} \tag{64}$$

where the mirror symmetries $m_x$ and $m_y$ are represented by $\pm\sigma_z$, such that the system satisfies $\sigma_z H(k_x, k_y, k_z)\sigma_z = H(-k_x, k_y, k_z) = H(k_x, -k_y, k_z)$. In solid state, such a model could be implemented by two bands formed by $p_x$ and $p_y$ atomic orbitals. We set

$$A = 2, \qquad B_1 = 1, \qquad B_2 = 1.5, \qquad D = 1.5, \qquad E = 1, \tag{65}$$

and keep $C$ as a tunable parameter.

Let us first investigate the Hamiltonian on the high symmetry planes $k_{x,y} \in \{0, \pi\}$ and on their intersections. For logical convenience, we start with $k_y \in \{0, \pi\}$ planes where the Hamiltonian reads

$$H(\mathbf{k}) = [A + B_1 \pm B_2 + B_1 \cos 2k_x - (B_2 \pm C)\cos k_x - D\cos k_z]\,\sigma_z \equiv d_z(\mathbf{k})\sigma_z, \tag{66}$$

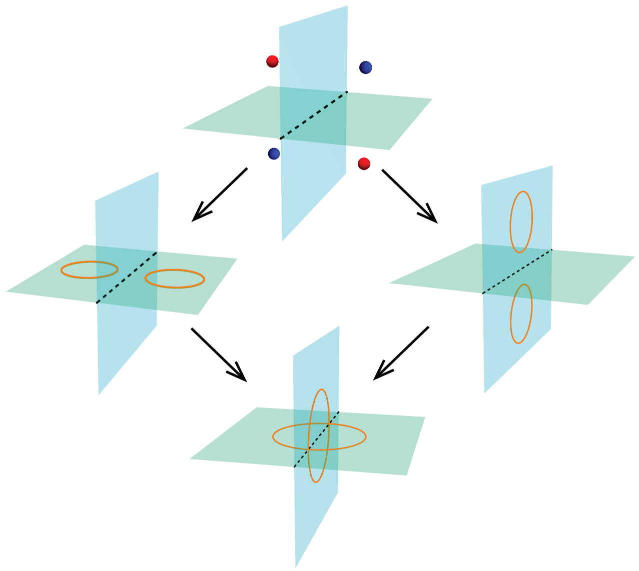

**Figure** S-6. Converting band-structure nodes of two-band models if the basis orbitals differ in eigenvalues of both $m_x$ and $m_y$ mirror symmetries, such as $p_x$ and $p_y$. The blue and green sheets indicate mutually perpendicular mirror-invariant planes. The presence of one Weyl point automatically implies the presence of three additional ones. Weyl points related by a mirror symmetry carry opposite chirality (red = positive, blue = negative). Symmetry-preserving evolution of the Hamiltonian can bring pairs of Weyl points of opposite chirality together at either one of the two mirror-invariant planes. Such a collision converts pairs of Weyl points into nodal loops due to the conservation of the second relative homotopy charge. Furthermore, the two obtained nodal loops can be brought to the symmetric line in the centre (cross-section of the mirror-invariant planes), where they fuse into a nodal chain. The resulting nodal chain carries $|n_{W2}| = 1$, and is expected to connect with four surface Fermi arcs to other objects in the surface Brillouin zone.

where the $\pm$ sign corresponds to the $k_y = 0$ vs. the $k_y = \pi$ plane. Assuming that $|(B_2 \pm C)/4B_1| < 1$, it is easy to check by calculating the derivatives that $d_z(\mathbf{k})$ reaches its minima at

$$(k_x^{\mathrm{min}}, k_z^{\mathrm{min}}) = \left(\pm \arccos\left(\frac{B_2 \pm C}{4B_1}\right), 0\right) \qquad \text{with the minimal value} \quad d_z^{\mathrm{min}} = -\frac{(B_2 \pm C)^2}{8B_1} + A - D \pm B_2. \tag{67}$$

For $C = 2.5$ inside the $k_y = 0$ plane, the minimal value is $d_z^{\mathrm{min}} = 0$ and there is only a single band touching point at $\mathbf{k} = (0,0,0)$. One may check that the contour of $d_z(\mathbf{k}) = 0$ in the $k_x = 0$ plane creates two nodal loops (one for $k_x > 0$ and one for $k_x < 0$), which touch at $\mathbf{k} = (0,0,0)$. This is a critical point of converting two nodal loops into a nodal chain along a high-symmetry line $(k_x, k_y) = (0,0)$.

The bulk nodal structures for $C = 2$ and $C = 3$ on the two sides of the critical point are plotted in Fig. 3(c) and Fig. 3(d) of the main text, respectively. One can see that as $C$ increases from 2 to 2.5, the two nodal loops in the $k_x = 0$ plane move towards each other until they collide. As $C$ increases from 2.5 to 3, the touching point grows into a nodal loop in the $k_y = 0$ plane and form a nodal chain centered at $(k_x, k_y) = 0$.

Note that there is an accidental symmetry of our Hamiltonian under transformation $(k_x, k_y) \to (\pi - k_y, \pi - k_x)$. Therefore, one expects a similar conversion to happen at the corner $(k_x, k_y) = (\pi, \pi)$. Indeed, as $C$ increases from 2 to 2.5, two nodal loops in the $k_y = \pi$ plane move towards each other, until they collide at $\boldsymbol{k} = (\pi, \pi, 0)$. For $C > 2.5$, the touching point grows into a nodal loop in the $k_x = \pi$ plane, such that a nodal chain is formed.

For the bulk-edge correspondence, we can compute the winding number $n_{W2}$ on a quarter-sphere centered at $\mathbf{k} = (0,0,0)$ using similar integration as in Eq. (62). One can set the integration surface as $\mathbf{k} = R(\sin\theta\cos\phi, \sin\theta\sin\phi, \cos\theta)$, where $R$ is chosen to be large enough to enclose the nodal structure centered at $\mathbf{k} = (0,0,0)$. Numerical evalution shows that

$$n_{W2} = \frac{1}{4\pi}\int_0^{\pi} d\theta \int_0^{\pi/2} d\phi \frac{\mathbf{d}\cdot(\partial_\theta \mathbf{d} \times \partial_\phi \mathbf{d})}{|\mathbf{d}|^3} = 1. \tag{68}$$

This leads to four Fermi arcs connecting the projection of the nodal structure at $\mathbf{k} = (0,0,0)$ to other nodes in the surface BZ.

We finally remark that the presented model can also realize the conversion of NLs into WPs, which completes the conversion scheme illustrated in Fig. S-6. One can start with the $C = 2$ case, where there are two NLs inside the $k_x = 0$ plane as well as two NLs inside the $k_y = \pi$ plane. One can increase $A$ and observe the shrinking of all the NLs. For $A = 2.75$, each NL ejects a pair of mirror-related Weyl points. In this process, the non-trivial charge is carried off by the Weyl points, while the NLs become

trivial. Further increasing $A$ to values larger than 3 removes the NLs from the spectrum, while carrying the WPs away from the symmetric planes. The described conversion into multiple WPs also manifestly reflects the non-trivial quadrupole character of the nodal structure.

### C. Lattice model exhibiting the conversion of Weyl points in the presence of $C_{2z}\mathcal{T}$ symmetry

We consider the lattice Hamiltonian

$$H(\mathbf{k}) = (-2\cos k_x - 2\cos k_y + 2\cos k_z + 2 - m)\sigma_x + \sin k_y \sigma_y + \sin k_x \sin k_z \sigma_z, \tag{69}$$

where $m$ is the only adjustable parameter. Model (69) is symmetric under $C_{2z}\mathcal{T}$ symmetry represented by $\sigma_x K$ (with $K$ being the complex conjugation). We further focus on the $C_{2z}\mathcal{T}$-invariant plane with $k_z = 0$. The expansion of the Hamiltonian up to quadratic order around $\mathbf{k} = \mathbf{0}$ is

$$H_{\text{eff.}}(\mathbf{k}) = (k_x^2 + k_y^2 - k_z^2 - m)\sigma_x + k_y\sigma_y + k_x k_z \sigma_z \tag{70}$$

Near the centre of the Brillouin zone $\mathbf{k} = \mathbf{0}$, there are two WPs at $(k_x, k_y, k_z) = (\pm\sqrt{m}, 0, 0)$ for $m > 0$ [with charges $(n_\text{C}, n_\text{H}) = (1, \pm 1)$], while there are two WPs at $(k_x, k_y, k_z) = (0, 0, \pm\sqrt{|m|})$ for $m < 0$ [both with charge $(n_\text{C}, n_\text{H}) = (1, 0)$]. The pseudospin configurations in Fig. 4(a-b) of the main text correspond to model (69) with $m = -2$ and $m = 2$, respectively. Note that both of the integer charges $n_\text{C}$ and $n_\text{H}$ are conserved in the conversion occurring at $m = 0$.

## V. NO STABLE FERMI ARCS FOR NODES IN SYSTEMS WITH $(\mathcal{PT})^2 = +1$ SYMMETRY

It is well understood that stable nodal lines can exist in three-dimensional $\mathcal{PT}$-symmetric models without spin-orbit interaction [7]. Under these circumstances, electrons are effectively spinless, such that $\mathcal{T}^2 = +\mathbf{1}$, which together with $\mathcal{P}^2 = +\mathbf{1}$ and $[\mathcal{P}, \mathcal{T}] = 0$ imply $(\mathcal{PT})^2 = +\mathbf{1}$. This locates such semimetals in nodal class AI [3]. By a suitable rotation of the basis, one can represent $\mathcal{PT}$ by the complex conjugation $K$, so that the single-particle Hamiltonian $H(\mathbf{k})$ is a real symmetric matrix at every $\mathbf{k} \in$ BZ. Expanding a minimal two-band Hamiltonian near a band touching results in an effective $2 \times 2$ real symmetric Hamiltonian $H(\mathbf{k}) = \epsilon(\mathbf{k})\mathbf{1} + d_x(\mathbf{k})\sigma_x + d_z(\mathbf{k})\sigma_z$. Two conditions $d_x(\mathbf{k}) = 0 = d_z(\mathbf{k})$ have to be fulfilled to close the band gap, which in 3D indeed facilitates nodal lines. The stability of such nodal lines follows from the homotopy group

$$\pi_1(M_\text{AI}) = \mathbb{Z}_2 \tag{71}$$

where $M_\text{AI} = \mathsf{O}(n+\ell)/\mathsf{O}(n)\times\mathsf{O}(\ell)$ is the corresponding space of gapped Hamiltonians, and $n, \ell$ indicate the number of occupied and unoccupied bands, respectively. Charge (71) corresponds to the quantized Berry phase on closed paths in $\mathbf{k}$-space.

Importantly, it was found by Ref. [7] that there is an *additional* $\mathbb{Z}_2$ charge associated with nodal loops protected by $\mathcal{PT}$ symmetry, which follows from the *second* homotopy group

$$\pi_2(M_\text{AI}) = \mathbb{Z}_2 \tag{72}$$

The topological charge following from (72) is commonly called the $\mathbb{Z}_2$ *monopole charge*. It can be calculated by studying the Wilson loop spectra on a sphere fully enclosing the nodal loop [3].

Topological invariants defined on a 2D manifold in BZ may imply Fermi arc states passing through the projection of the manifold inside the surface BZ (SBZ). The simplest such an example occurs in Weyl semimetals [17], where a Chern number can be defined on a sphere enclosing a WP. This Chern number is related to the surface Fermi arcs emanating from the projection of the bulk WPs inside the SBZ. A more complex case has been discussed for two-band mirror-symmetric models in Fig. S-5. Let us review here the original argument for the bulk-boundary correspondence as it appeared in the context of Weyl points in Ref. [17]. The argument assumes a soft interface with Hamiltonian parameters slowly interpolating between a topological semimetal and a normal insulator.

We assume that a topological semimetal phase is realized for $x > 0$, while a normal insulator exists for $x < 0$. We can think of a region of size $L$ inside the normal insulator as indicated by the dashed box in Fig. S-7(a). Assuming that $L$ is much longer than the lattice constant and that the system inside the region has an approximate translational invariance, we may consider a “local” Bloch Hamiltonian $H(\mathbf{k}, x)$. As $x$ varies from $-\infty$ to $+\infty$, $H(\mathbf{k}, x)$ smoothly interpolates between the Hamiltonian of the normal insulator and the Hamiltonian of the topological semimetal. For a given $x$, one can find the band structure of $H(\mathbf{k}, x)$ in the 3D BZ. Let us assume that there is a a non-trivial topological charge $Q \neq 0$ on a gapped manifold $M$ in the topological semimetal. The topological charge may be well-defined only in the presence of some symmetry group $G$, so we require the semiclassical Hamiltonian $H(\mathbf{k}, x)$ to preserve the symmetry $G$ for every $x \in \mathbb{R}$. Considering the adiabatic evolution of Hamiltonian $H(\mathbf{k}, x)$

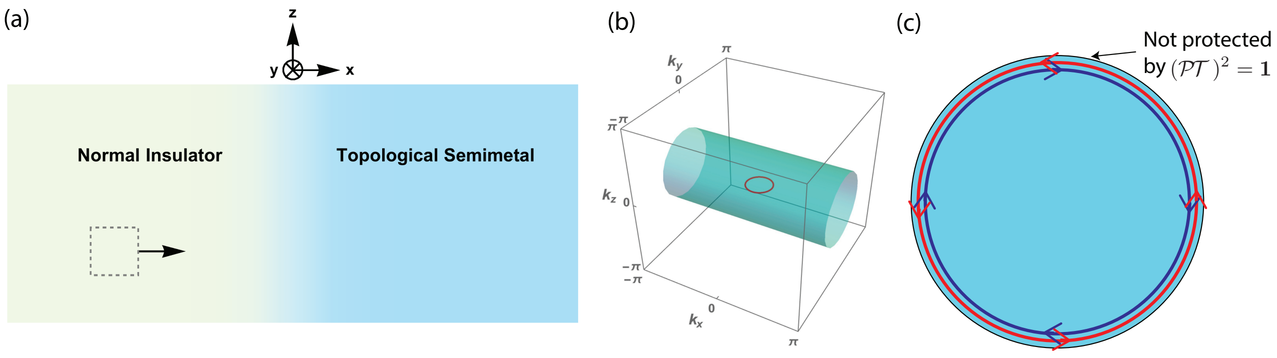


**Figure** S-7. Illustration of the argument for the bulk-boundary correspondence. (a). A sketch of the setting. We consider a soft interface between a normal insulator and a topological semimetal, such that one can consider the dashed region to have a well-defined "local" Bloch Hamiltonian $H(\mathbf{k}, x)$ that varies slowly with position $x$. We assume there is a two-dimensional manifold $M \subset$ BZ supporting a topological charge taking different values in the two phases. Then the spectral gap of $H(\mathbf{k}, x)$ must close at some $x_0$ and $\mathbf{k} \in M$. This corresponds to a surface state. (b-c). The absence of Fermi arcs in nodal-line semimetals with $\mathcal{PT}$ symmetry. (b) We consider a cylinder enclosing a nodal loop with a non-trivial $\mathbb{Z}_2$ monopole (72), and interpret the cylinder as describing a two-dimensional system. (c) Assuming that the monopole charge creates an edge mode in the two-dimensional system, we deduce that $\mathcal{PT}$ symmetry implies the existence of a counter-propagating edge mode. This follows because $\mathcal{PT}$ flips the chirality. Since there is no symmetry to protect the crossing of the two edge modes, a gap generically opens while preserving the $\mathcal{PT}$ symmetry of the system.

on $M$, we deduce that the topological charge on $M$ *changes* between $x = -\infty$ to $x = +\infty$ from $Q$ (in the semimetal) to 0 (in the insulator). Therefore, $H(\mathbf{k}, x)$ has to close the bulk gap for some $x_0 \in \mathbb{R}$ at some $\mathbf{k} \in M$ to accommodate for the change of the topological quantity. We thus deduce the existence of a surface state at $x_0$ with a momentum lying on the projection of $M$ inside the SBZ.

However, this argument *breaks down* for the $\mathcal{PT}$-protected $\mathbb{Z}_2$ monopole (72). The crucial loophole here is that the semiclassical Hamiltonian $H(\mathbf{k}, x)$ does *not* have $\mathcal{PT}$ symmetry since $\mathcal{PT}$ flips $x \mapsto -x$. Consequently, the intermediate Hamiltonians $H(\mathbf{k}, x)$ don't have a well-defined topological charge on the manifold $M$, so there is no implied conservation rule, and no surface states at intermediate $x_0 \in \mathbb{R}$. Alternatively, one can consider the gapped subsystem on a cylinder enclosing the band-structure node, which projects onto a circle in the SBZ [Fig. S-7(b)]. If this gapped two-dimensional subsystem has one branch of chiral modes $\psi_L$, the $\mathcal{PT}$ symmetry requires another branch of counter-propagating chiral modes $\psi_R$ because $\mathcal{PT}$ symmetry flips the chirality [Fig. S-7(c)]. The coupling between $\psi_L$, $\psi_R$ can open a gap in the surface states without breaking the $\mathcal{PT}$ symmetry. This is the general situation in the absence of fine-tuning.

Ref. [20] studied the surface Fermi arcs in real Dirac semimetal that exhibits point nodes with non-trivial $\mathbb{Z}_2$ monopole charge (72) at the Fermi energy. Here, we show that these Fermi arc states are not stable against $\mathcal{PT}$-invariant perturbations. The lattice model of Ref. [20] reads

$$H_0(k) = 2t_x \sin k_x \sigma_1 \otimes \tau_2 + 2t_y \sin k_y \sigma_2 \otimes \tau_0 + [m - f(k)]\sigma_3 \otimes \tau_0, \tag{73}$$

where $f(k) = \alpha_+(\cos k_x + \cos k_z) + \alpha_- \cos k_y$, $\sigma_i$ and $\tau_i$ are two sets of Pauli matrices, and the $\mathcal{PT}$ symmetry is represented as $\mathcal{PT} = \sigma_3 K$. In the parameter region with

$$t_x \neq 0, \qquad 0 < \frac{m - \alpha_-}{2\alpha_+} < 1 \qquad \text{and} \qquad \frac{m + \alpha_-}{2\alpha_+} > 1, \tag{74}$$

the band structure exhibits a pair Dirac points. As shown in Ref. [20], both Dirac points carry a non-trivial value of the $\mathbb{Z}_2$ monopole. For a surface termination in the $y$ direction, we reproduce a doubly degenerate Fermi arc connecting the projections of the two Dirac points (see surface spectrum in Fig. S-8(a)) as reported in Ref. [20]. This is not surprising, since rotating $\tau_1 \mapsto \tau_2 \mapsto \tau_3 \mapsto \tau_1$ brings (73) into a block structure corresponding to two Weyl semimetals that are not coupled. The doubly degenerate states on the Fermi arc are eigenstates of operator $\chi = \sigma_1 \otimes \tau_2$ with eigenvalues $+1$ and $-1$[21]. Therefore, a perturbation term proportional to $\tau_1$ or $\tau_3$, which couples two states with $\chi = \pm 1$, will generically gap out the Fermi arc. In the simulation, we add the following term,

$$H(k) = H_0(k) + 2t_z \cos k_z \tau_3, \tag{75}$$

which preserves $\mathcal{PT}$ symmetry. When we turn on the $t_z$ term of Eq. (75), the Dirac points may become nodal lines in generic situations. In Fig. S-8(b), we fine-tune the Dirac points to be at $k_z = \pm\pi/2$, such that the extra term vanishes exactly at the Dirac

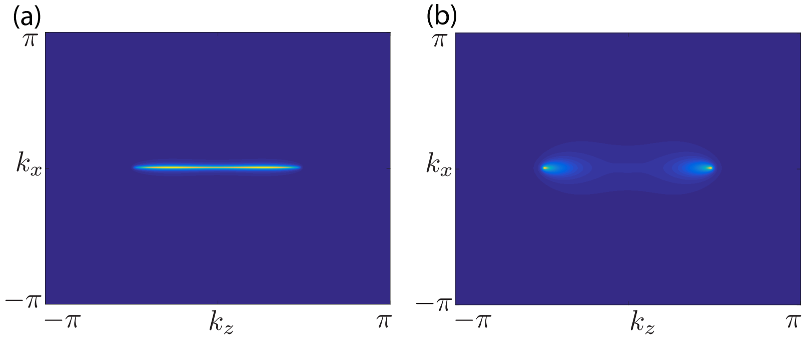


**Figure** S-8. (a) The density of states at Fermi energy for lattice model (73) with $\alpha_+ = 0.6$, $\alpha_- = 0.4$, $m = 1$, $t_x = 0.2$ and $t_y = 0.5$. We observe a (two-fold degenerate) Fermi arc connecting the projections of a pair of Dirac points. (b) Including an additional term (75) with $t_z = 0.09$ keeps the Dirac points while removing the Fermi-arc states.

points and the nodal lines are shrunk to the two Dirac points. In this situation, the Dirac points are still present but the Fermi arc disappears from the SBZ, because the $t_z$ term couples two states in the unperturbed Fermi arc.

We remark that although $\mathcal{PT}$ symmetry cannot protect Fermi-arc surface states, $\mathcal{PT}$ can indeed protect the drumhead surface states. This follows by considering the charge polarization interpretation of the Zak phase [22, 23]. We shall illustrate this idea on the (100) surface. Since the (100) surface preserves translations in the $y$ and $z$ directions, we can consider an effectively one-dimensional subsystem with fixed $k_y$ and $k_z$. When the subsystem is gapped, the $\mathcal{PT}$ symmetry quantizes the Zak phase $\theta(k_y, k_z)$ to 0 or $\pi$, which can be interpreted as a topological $\mathbb{Z}_2$ invariant. If we consider a situation where $\theta(k_y, k_z) = 0$ deep inside the normal insulator at $x < 0$ while $\theta(k_y, k_z) = \pi$ deep inside the topological semimetal at $x > 0$, then the total charge accumulation at the surface is:

$$Q_{\text{surface}} = \int_{-\infty}^{\infty} dx \partial_x P_x = \frac{1}{2\pi} \int_{-\infty}^{\infty} \partial_x \theta(k_y, k_z, x) = \frac{1}{2} \tag{76}$$

As previously studied in Ref. [24], the half-charge corresponds to the existence of a zero mode. We can understand the stability of the zero mode, because for such a one dimensional subsystem the $\mathcal{PT}$-related partner of the boundary mode lies on the opposite end of the system. Therefore, local single-electron operators cannot open a gap.

We finally comment here again on the topological invariant on 2D manifolds that we introduced for mirror-symmetric two-band systems in Sec. III B. Here, the semiclassical argument [summarized in Fig. S-5(b,c)] works, because we can find symmetry-preserving surfaces. For example, in the presence of $m_z$ symmetry, the coordinate $x$ is left invariant by $m_z$, such that the semi-classical Hamiltonian at $x$ is also invariant under $m_z$: $H(k_x, k_y, k_z, x) \to m_z H(k_x, k_y, -k_z, x) m_z^{-1}$. For this reason, mirror symmetry can protect Fermi-arc surface states.

## VI. GENERALIZATION TO MULTI-BAND MODELS

We argued that some of the new topological invariants introduced in Sec. III cease to exist in multi-band models. However, nodal lines are protected by the mirror symmetry and the WPs are protected by the Chern number, meaning that both nodal structures are resilient to the inclusion of additional bands. In this section, we investigate how the *conversion rule* between the two species of nodes in the presence of a mirror-symmetry is *modified* in the presence of additional bands.

We illustrate the idea by adding a single flat band at the bottom of an effective Hamiltonian,

$$H(\mathbf{k}) = \sum_{n=1,2} E_{n\mathbf{k}} |\mathbf{k}, n\rangle\langle\mathbf{k}, n| + \Delta|\Delta, \mathbf{k}\rangle\langle\Delta, \mathbf{k}| + \lambda V, \tag{77}$$

where $V$ represents symmetry-compatible coupling of the flat band to the original two bands, $\Delta$ is the energy of the flat band, and $\lambda$ is a small parameter. From the perturbation theory, the correction to $E_{n\mathbf{k}}$ is of order $O(\frac{\lambda^2}{E_{n\mathbf{k}}-\Delta})$.

Let us consider the case, where a pair of WPs convert into a NL in a mirror-invariant plane. When we are *far* from the critical point (i.e. either the WPs are far away from each other, or the NL is large enough), then the correction would slightly change the position of the WPs or deform the NL. On the other hand, *near* the critical point (i.e. either the WPs are close together, or the NL is very small), the correction might harmfully meddle with the critical point of the topological phase transition. In other words, we expect the perturbation to expand the critical point of the conversion into a narrow *transition regime*, where the conversion rule can be violated. Within this regime, we might observe *both* the NL and the WPs, as well as *none* of them. The range of this transition regime is set by the energy scale $O(\frac{\lambda^2}{E_{n\mathbf{k}}-\Delta})$.

One can study the intermediate regime on an explicit model, such as the $m_z$-symmetric

$$H(\mathbf{k}) = \begin{pmatrix} k_z^2 - k_x^2 - k_y^2 - M & k_z(k_x - ik_y) & \lambda b k_z \\ k_z(k_x + ik_y) & -(k_z^2 - k_x^2 - k_y^2 - M) & \lambda a \\ \lambda b k_z & \lambda a & -\Delta \end{pmatrix}. \tag{78}$$

Here, the upper-left 2×2 block corresponds to the original model, which exhibits a conversion of a NL (for $M < 0$) into a pair of WPs (for $M > 0$). We further included a flat band with negative energy $-\Delta$, which couples to the original two orbitals of the effective Hamiltonian with matrix elements $a$ and $bk_z$. The parameter $\lambda$ corresponds to turning on the perturbation, and ranges from 0 to 1. The mirror operator in this basis is $m_z = (1, -1, -1)$, and the coupling terms are chosen such that they preserve the $m_z$-symmetry. Since the Fermi velocity near the nodes of unperturbed model (78) is $v_\mathrm{F} \sim \sqrt{|M|}$ and because the separation of the nodes is $\delta k \sim \sqrt{|M|}$, the relevant energy scale for the topological phase transition is $\delta k\, v_\mathrm{F} \sim |M|$. This energy scale has to be compared to the perturbative correction to the band energies, therefore [ignoring the the factors $a, b$ in Eq. (78)] we expect the transition regime for $|M| \lesssim \lambda^2/\Delta$ [Fig. S-9].

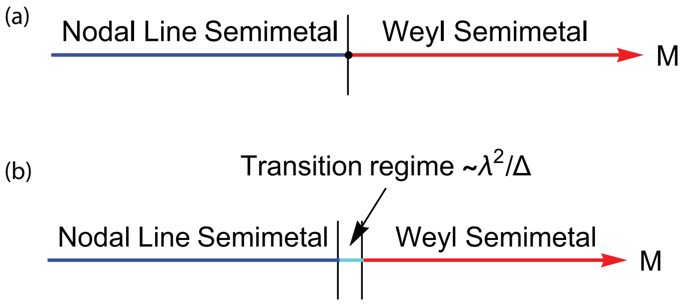


**Figure** S-9. (a) For $\lambda = 0$, the two bands with higher energy are captured by a strictly two-band model, which produces a nodal-line (Weyl) semimetal for $M < 0$, ($M > 0$). A conversion between the two species of nodes occurs at $M = 0$. (b) We include a coupling of strength $\lambda$ to a third band at large negative energy $-\Delta$. This broadens the critical point into a transition regime of the indicated width. Within this regime, the (dis)appearance of NL/WPs occurs asynchronously.

---


[1] A. Hatcher, *Algebraic Topology* (Cambridge University Press, Cambridge, 2002).
[2] N. D. Mermin, Rev. Mod. Phys. **51**, 591 (1979).
[3] T. Bzdušek and M. Sigrist, Phys. Rev. B **96**, 155105 (2017).
[4] A. T. Lundell, Lect. Notes Math. **1509**, 250 (1992).
[5] zdus, "Conditions for the second homotopy group to be abelian," MathOverflow (2018), (version: 2018-02-27).
[6] Wikipedia contributors, "Direct product of groups — Wikipedia, The Free Encyclopedia," (2017).
[7] C. Fang, Y. Chen, H.-Y. Kee, and L. F. Fu, Phys. Rev. B **92**, 081201(R) (2015).
[8] M. Fischer, M. Sigrist, and D. F. Agterberg, ArXiv e-prints (2018), arXiv:1803.06504.
[9] A. Kitaev, AIP Conf. Proc. **1134**, 22 (2009).
[10] T. Bzdušek and S.-C. Zhang, in preparation (2018).
[11] T. Bzdušek, Q.-S. Wu, A. Rüegg, M. Sigrist, and A. A. Soluyanov, Nature **538**, 75 (2016).
[12] T. Oh and B.-J. Yang, ArXiv e-prints (2017), arXiv:1709.06796.
[13] Z. Wang, D. Gresch, A. A. Soluyanov, W. Xie, S. Kushwaha, X. Dai, M. Troyer, R. J. Cava, and B. A. Bernevig, Phys. Rev. Lett. **117**, 056805 (2016).
[14] A. Altland and M. R. Zirnbauer, Phys. Rev. B **55**, 1142 (1997).
[15] A. P. Schnyder, S. Ryu, A. Furusaki, and A. W. W. Ludwig, Phys. Rev. B **78**, 195125 (2008).
[16] freakish, "Finding a group with a prescribed normal subgroup and quotient group," Mathematics Stack Exchange (2018), (version: 2018-02-28).
[17] X. Wan, A. M. Turner, A. Vishwanath, and S. Y. Savrasov, Phys. Rev. B **83**, 205101 (2011).
[18] P. Hosur and X. Qi, C. R. Phys. **14**, 857 (2013).
[19] Y. Wang and P. Ye, Phys. Rev. B **94**, 075115 (2016).
[20] Y. Zhao and Y. Lu, Phys. Rev. Lett. **118**, 056401 (2017).
[21] The choice of operator $\chi$ depends on the surface termination as well as the direction of Fermi arc. As shown by Ref. [25], the operator $\chi$ should be the gamma matrix of the effective Dirac Hamiltonian near the Dirac point, coupling to the momentum perpendicular to both the Fermi arc direction and the surface termination direction.
[22] J. Zak, Phys. Rev. Lett. **62**, 2747 (1989).

[23] R. D. King-Smith and V. David, Phys. Rev. B **47**, 1651(R) (1993).
[24] P. Delplace, D. Ullmo, and G. Montambaux, Phys. Rev. B **84**, 195452 (2011).
[25] E. Witten, arXiv preprint arXiv:1510.07698 (2015).
